# Supplementary material for: DPAUC: Differentially Private AUC Computation in Federated Learning
Source: arXiv:2208.12294 source file (2022-12-07)
Supplement: Supplementary file 1 [file algorithm_dpauc_lap.tex]

%%%%% Algorithm 
% \begin{comment}
 \begin{algorithm}[ht!]
\caption{\ourapplap{}}\label{alg:clients_server_cal_auc_localdp}
\KwData{The $K$ clients are index by $k$. Each client $C_k$ has  data $D_k$ with $(X_k, Y_k)$ where $Y_k \in [0,1]$. Model $f$. Decision boundaries $\Theta$.}
\KwResult{$\text{AUC}$}

\textbf{ // Clients Execute}

     \For{each client $C_k$}{
        \For{each data point $(x_i, y_i) \in (X_k, Y_k
        )$}{
        Calculate the corresponding prediction score $s_i^k = f(x_i)$
        }
        
    \For{each  $\theta \in \Theta$}{
        Calculate the corresponding four local statistics: $\text{TP}_k^\theta$, $\text{TN}_k^\theta$, $\text{FP}_k^\theta$, and $\text{FN}_k^\theta$
        }
    \For{each  $\theta \in \Theta$}{
        Add DP noise to the four local statistics: 

        $\text{TP}_k^{\theta '} = \text{TP}_k^\theta + \textsf{Lap}(1/\epsilon_{\text{TP}}) $ 
        
        $\text{FP}_k^{\theta '} = \text{FP}_k^\theta + \textsf{Lap}(1/\epsilon_{\text{FP}}) $
        
        $\text{TN}_k^{\theta '} = \text{TN}_k^\theta + \textsf{Lap}(1/\epsilon_{\text{TN}}) $
        
        $\text{FN}_k^{\theta '} = \text{FN}_k^\theta + \textsf{Lap}(1/\epsilon_{\text{FN}}) $

        }

    Sends the noisy local statistics to the Server.
    }

\textbf{ // Server Executes}

\For{each  $\theta \in \Theta$}{
Aggregates the noisy statistics from all the clients: 

$\text{TP}^{\theta} = \sum_{k=1}^K \text{TP}_k^{\theta '}$

$\text{TN}^{\theta} = \sum_{k=1}^K \text{TN}_k^{\theta '}$

$\text{FP}^{\theta} = \sum_{k=1}^K \text{FP}_k^{\theta '}$

$\text{FN}^{\theta} = \sum_{k=1}^K \text{FN}_k^{\theta '}$ 
}

\For{each  $\theta \in \Theta$}{
Computes the corresponding $\text{TPR}$ and $\text{FPR}$: 

$\text{TPR}^\theta = \frac{\text{TP}^\theta}{\text{TP}^\theta + \text{FN}^\theta}$

$\text{FPR}^\theta = \frac{\text{FP}^\theta}{\text{FP}^\theta + \text{TN}^\theta}$
}

The server plots TPR (x-axis) vs. FPR (y-axis) over all possible thresholds $\theta$ and computes the area under the corresponding curve as the final AUC.
 
\end{algorithm}
% \end{comment}
