# Supplementary material for: DPAUC: Differentially Private AUC Computation in Federated Learning
Source: arXiv:2208.12294 source file (2022-12-07)
Supplement: Supplementary file 2 [file appendix_fedauc.tex]

\section{Appendix}
\label{sec:appendix}

\textbf{Appendix Outline:}

Section ~\ref{sec:illustration_rr}: Illustration of our proposed \ourapp{} with randomized response.

Section ~\ref{sec:illustration_laplace}: Illustration of our proposed \ourapp{} with Gaussian or Laplace mechanism

Section ~\ref{sec:algo_rr_appendix}: Algorithm  ~\ref{alg:clients_flipping_labels}: Clients leverages randomized response to flip labels with $\epsilon$-LabelDP guarantee

Section ~\ref{sec:algorithm_noisy_auc_appendix} : Algorithm ~\ref{alg:clients_server_cal_auc}: Sever computes noisy AUC with clients' local flipped labels

Section ~\ref{sec:clean_auc_appendix}: Algorithm ~\ref{alg:real_auc_from_corr}: Server computes the clean/final AUC

Section ~\ref{sec:algorithm_noisy_auc_lap_appendix}: Algorithm ~\ref{alg:clients_server_cal_auc_2}: Sever computes noisy AUC with clients' local labels

Section ~\ref{sec:auc_probabilistic_view}: Computing  AUC from a probabilistic perspective

Section ~\ref{sec:utility_rr}: Utility analysis of RR

Section ~\ref{sec:auc_probabilistic_view}:  Computing  AUC from a probabilistic perspective

Section ~\ref{sec:utility_rr}: Utility analysis of RR

Section ~\ref{sec:std_auc_different_alpha_non_iid_appendix}: Standard deviation of AUC with different DP budget allocation $\alpha$ in the Non-IID setting

Section ~\ref{sec:ortho_adaptive_iid_appendix}:  Orthogonalizatin vs. Adaptive allocation in the IID setting

Section ~\ref{sec:noisy_auc_rr_appendix}: Noisy AUC computed by Randomized Response without debiasing

Section ~\ref{sec:more_results_criteo_rr_appendix}: More results of Randomized Responses on Criteo dataset

Section ~\ref{sec:var_auc_globallaplace}: Variance of AUC estimated by GlobalLaplace

Section ~\ref{sec:utility_analysis_locallap_appendix}: Utility analysis of LocalLaplace

Section ~\ref{sec:estimate_pi}: Estimate $\pi'$

Section ~\ref{sec:compare_all_methods_auc_appendix}: Table ~\ref{tab:std_auc_w_noisy_P_and_N}: std of AUC estimated different methods: RR vs. GlobalLaplace vs. LocalLapace with adaptive budget allocation

Section ~\ref{sec:sorting_module}: Privacy analysis of prediction scores 

Section ~\ref{sec:dist_of_local_beta}: Figure: ~\ref{fig:dist_of_local_beta}: Distribution of local $\beta$

Section ~\ref{sec:computation_resources}: Computational resources

\clearpage

\section{Illustration of our proposed \ourapp{} with randomized response}
\label{sec:illustration_rr}

Illustration of our proposed \ourapp{} with randomized response can be seen in Figure ~\ref{fig:fedauc_illustration_rr}.

\begin{figure*}[ht!]% \vspace{-0.1in}
  \centering
  \includegraphics[width=1.0\linewidth]{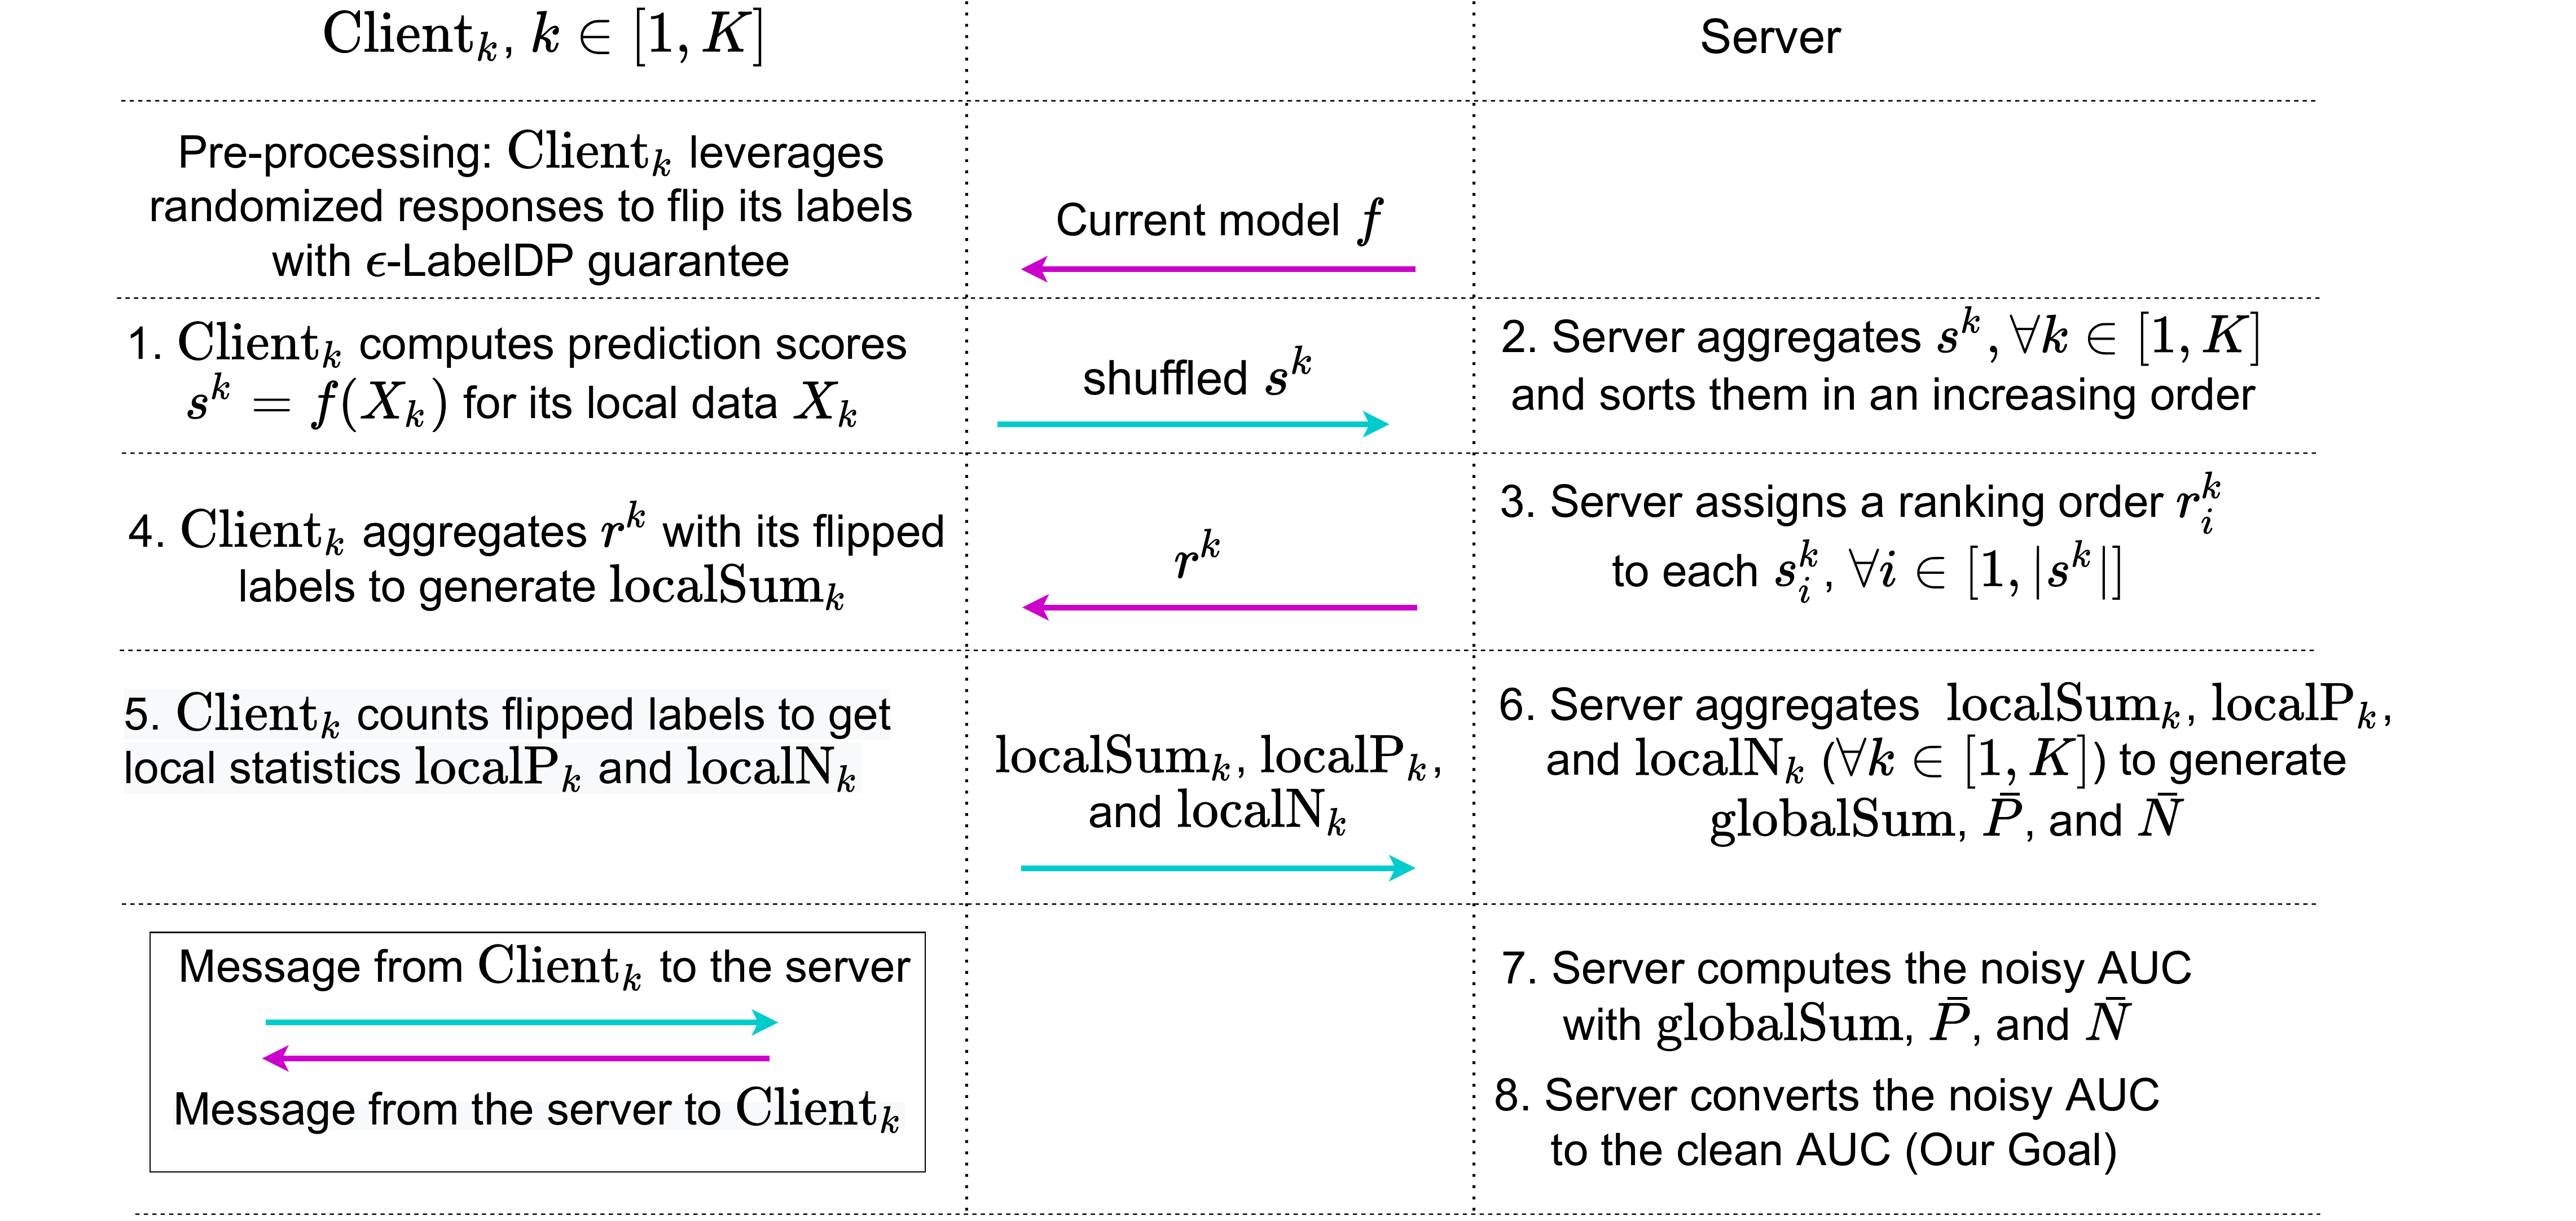}
  \caption{Illustration of our proposed \ourapp{} with randomized response.}
 \label{fig:fedauc_illustration_rr} 
 \end{figure*}
 
\section{Illustration of our proposed \ourapp{} with Gaussian or Laplace mechanism}
\label{sec:illustration_laplace} 

An illustration of our proposed \ourapp{} with Gaussian or Laplace mechanism can be seen in Figure ~\ref{fig:fedauc_illustration_lap}.

\begin{figure*}[ht!]% \vspace{-0.1in}
  \centering
  \includegraphics[width=1.0\linewidth]{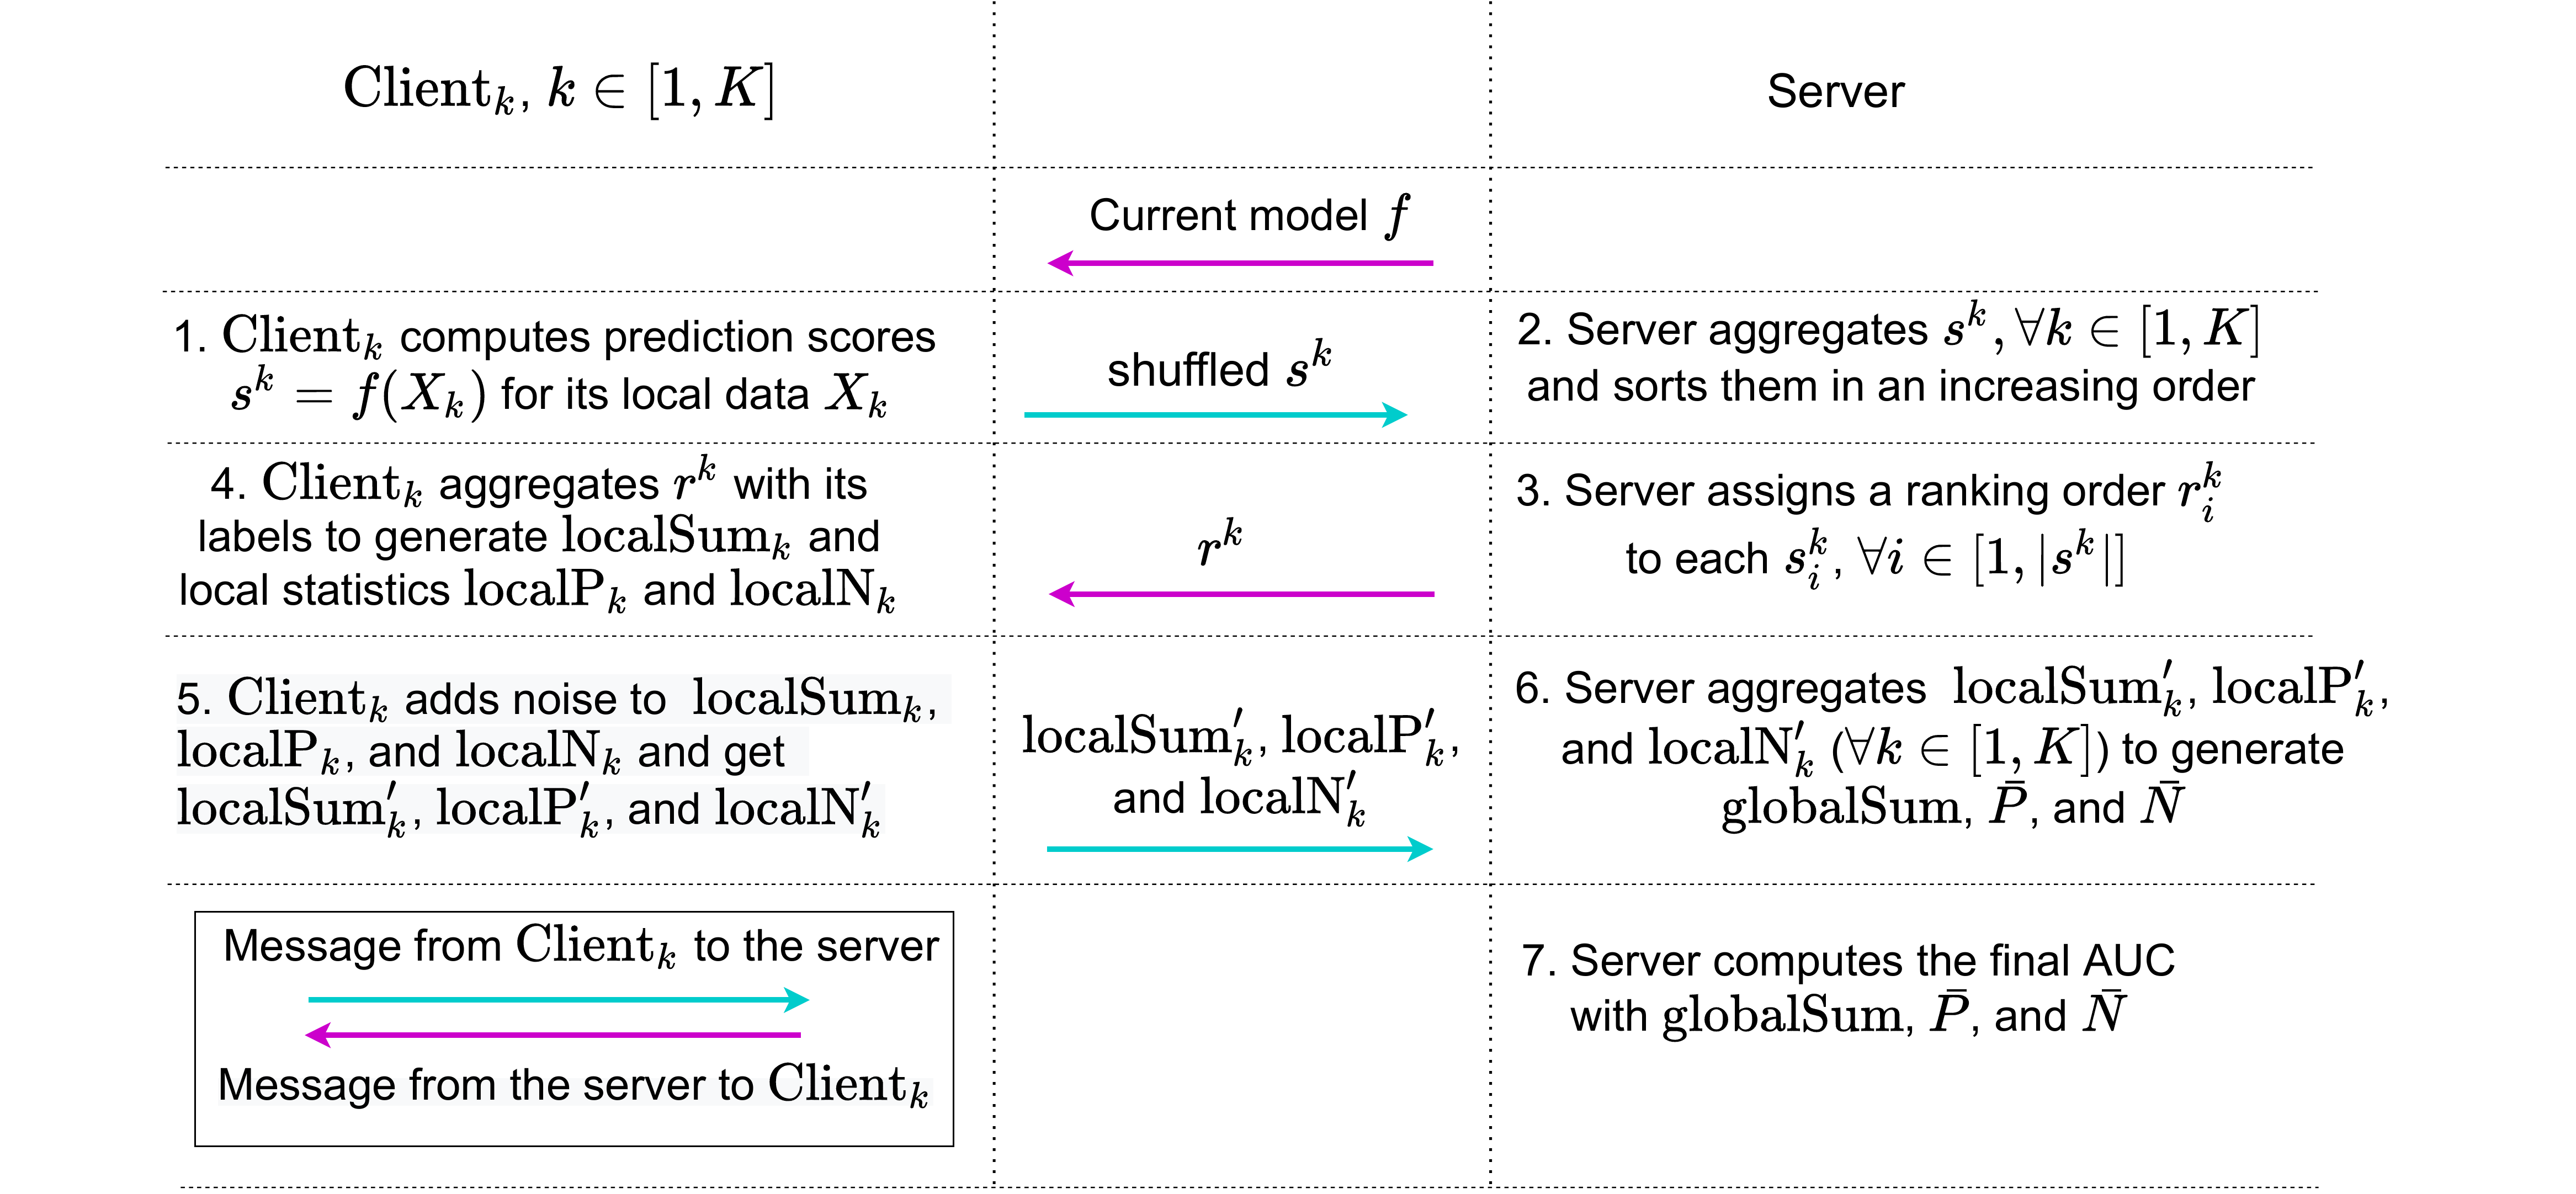}
  \caption{Illustration of our proposed \ourapp{} with Gaussian or Laplace mechanism.}
 \label{fig:fedauc_illustration_lap} 
 \end{figure*}

\section{Algorithm  ~\ref{alg:clients_flipping_labels}: Clients leverages randomized response to flip labels with $\epsilon$-LabelDP guarantee}
\label{sec:algo_rr_appendix}

Algorithm ~\ref{alg:clients_flipping_labels} shows how clients leverages randomized response to flip labels with $\epsilon$-LabelDP guarantee.

\begin{algorithm}[ht!]
\caption{Clients leverages randomized response to flip labels with $\epsilon$-LabelDP guarantee}\label{alg:clients_flipping_labels}
\KwData{The $K$ clients are index by $k$. Each client $C_k$ has data $D_k$ with $(X_k, Y_k)$ where $Y_k \in [0,1]$. Privacy budget $\epsilon$.}
\KwResult{Each client $C_k$ will have noisy data $D_k'$ with $\epsilon$-LabelDP guarantee}
 \For{each client $C_k$}{
    \For{each data point $(x_i, y_i) \in (X_k, Y_k)$}{
    replace $y_i$ by $\tilde{y_i}$ with randomized response as defined in equation ~\ref{eq:rr}.
    }
}
\end{algorithm}

\section{Algorithm ~\ref{alg:clients_server_cal_auc}: Sever Computes Noisy AUC with Clients' Local Flipped Labels}
\label{sec:algorithm_noisy_auc_appendix}

Algorithm ~\ref{alg:clients_server_cal_auc} shows how sever compute the noisy AUC with clients' local flipped labels.

\begin{algorithm}[ht!]
\caption{Sever Computes Corrupted AUC with Clients' Local Flipped Labels}\label{alg:clients_server_cal_auc}
\KwData{The $K$ clients are index by $k$. Each client $C_k$ has noisy data $D_k'$ with $(X_k, Y_k')$ where $Y_k' \in [0,1]$. Model $f$.}
\KwResult{Corrupted AUC: $\text{AUC}^{D_\text{noisy}}$}

\textbf{ // Clients Execute}

     \For{each client $C_k$}{
        \For{each data point $(x_i, y_i') \in (X_k, Y_k'
        )$}{
        Calculate the corresponding prediction score $s_i^k = f(x_i)$
        }
     Send all prediction scores $s^k$ to the server.
    }

\textbf{ // Server Executes}

Aggregate all the prediction scores and sort them in an increasing order.

Each prediction score $s_i^k$ ($i \in [1, M]$) will be assigned a ranking order $r_i^k$ as described in Section ~\ref{sec:computing_auc_ranking}.

Sends each ranking order $r_i^k$ back to the corresponding client $C_k$ which owns $s_i^k$.

\textbf{ // Clients Execute}
    
     \For{each client $C_k$}{
     
     $\text{localSum}_k, \text{localP}_k, \text{localN}_k  =  0, 0, 0 $

    \For{each data point $(x_i, y_i') \in (X_k, Y_k')$}{
        $\text{localSum}_k += r_i^k * y_i'$
        
        \eIf{$y_i' == 1$}{
            $\text{localP}_k  += 1$
                        }
            {
            $\text{localN}_k  += 1$
            }
        }
     $C_k$ sends $\text{localSum}_k$, $ \text{localP}_k$, and $\text{localN}_k$ to the server.
    }

\textbf{ // Server Executes}

// Server aggregates all the $\text{localSum}_k$, $ \text{localP}_k$, and $\text{localN}_k$.

$\text{globalSum} = \sum_{k}^K  \text{localSum}_k$

$\bar{P} = \sum_{k}^K \text{localP}_k$

$\bar{N} = \sum_{k}^K \text{localN}_k$

$\text{AUC}^{D_{\text{noisy}}} = ({\text{globalSum} - {\bar{P}(\bar{P}-1)}/{2}}) / ({\bar{P}\bar{N}}$)

\end{algorithm}

\section{Algorithm ~\ref{alg:real_auc_from_corr}: Server computes the clean/final AUC}
\label{sec:clean_auc_appendix}

Algorithm ~\ref{alg:real_auc_from_corr} shows how the server compute the clean/final AUC.

\begin{algorithm}[ht!]
\caption{Server computes the clean/final AUC}\label{alg:real_auc_from_corr}
\KwData{Corrupted AUC $\text{AUC}^{D_{\text{noisy}}}$, $\bar{P}$, $\bar{N}$, LabelDP budget $\epsilon$}
\KwResult{$\text{AUC}^{D_{\text{clean}}}$}

\textbf{ // Server Executes}

$\rho_{+} = \rho_{-} = \frac{1}{1+ e^{\epsilon}}$

$P' = \frac{\bar{P}(1-\rho_{-}) - \bar{N}\rho_{-}}{1-\rho_{+}-\rho_{-}}$

$N'= \bar{P}+\bar{N}-P'$

$\pi' = \frac{P'}{P' + N'}$

$\alpha = \frac{(1-\pi') \rho_{-}}{\pi(1-\rho_{+}) + (1-\pi')\rho_{-}}$

$\beta = \frac{\pi' \rho_{+}}{\pi' \rho_{+} + (1-\pi')(1-\rho_{-})}$
    
$ \text{AUC}^{D_{\text{clean}}}  =  \frac{\text{AUC}^{D_{\text{noisy}}} - \frac{\alpha+\beta}{2}}{1-\alpha-\beta}    $
\end{algorithm}

\section{Algorithm ~\ref{alg:clients_server_cal_auc_2}: Sever Computes Noisy AUC with Clients' Local Labels}
\label{sec:algorithm_noisy_auc_lap_appendix}

Algorithm ~\ref{alg:clients_server_cal_auc_2} shows how server compute noisy AUC with clients' local labels.

 \begin{algorithm}[ht!]
\caption{Sever Computes Noisy AUC with Clients' Local  Labels}\label{alg:clients_server_cal_auc_2}
\KwData{The $K$ clients are index by $k$. Each client $C_k$ has  data $D_k$ with $(X_k, Y_k)$ where $Y_k \in [0,1]$. Model $f$.}
\KwResult{AUC: $\text{AUC}$}

\textbf{ // Clients Execute}

     \For{each client $C_k$}{
        \For{each data point $(x_i, y_i) \in (X_k, Y_k
        )$}{
        Calculate the corresponding prediction score $s_i^k = f(x_i)$
        }
     Send all prediction scores $s^k$ to the server.
    }

\textbf{ // Server Executes}

Aggregate all the prediction scores and sort them in an increasing order.

Each prediction score $s_i^k$ ($i \in [1, M]$) will be assigned a ranking order $r_i^k$ as described in Section ~\ref{sec:computing_auc_ranking}.

Sends each ranking order $r_i^k$ back to the corresponding client $C_k$ which owns $s_i^k$.

\textbf{ // Clients Execute}
    
     \For{each client $C_k$}{
     
     $\text{localSum}_k, \text{localP}_k, \text{localN}_k  =  0, 0, 0 $

    \For{each data point $(x_i, y_i') \in (X_k, Y_k')$}{
        $\text{localSum}_k += r_i^k * y_i$
        
        \eIf{$y_i == 1$}{
            $\text{localP}_k  += 1$
                        }
            {
            $\text{localN}_k  += 1$
            }
        }
        
      $\text{localSum}_k'$ = $\text{localSum}_k$ + noise
      
      $\text{localP}_k'$ = $ \text{localP}_k$ + noise
      
      $\text{localN}_k$ = $|Y_k| - \text{localP}_k'$ 
      
     $C_k$ sends $\text{localSum}_k'$, $ \text{localP}_k'$, and $\text{localN}_k'$ to the server.
    }

\textbf{ // Server Executes}

// Server aggregates all the $\text{localSum}_k'$, $ \text{localP}_k'$, and $\text{localN}_k'$.

$\text{globalSum} = \sum_{k}^K  \text{localSum}_k'$

$\bar{P} = \sum_{k}^K \text{localP}_k'$

$\bar{N} = \sum_{k}^K \text{localN}_k'$

$\text{AUC} = ({\text{globalSum} - {\bar{P}(\bar{P}-1)}/{2}}) / ({\bar{P}\bar{N}}$)

\end{algorithm}

\section{Computing  AUC from a probabilistic perspective}
\label{sec:auc_probabilistic_view}

In a binary classification problem, given a threshold $\theta$, a predicted score $s_i$ is predicted to be $1$ if $s_i \ge \theta$. Given the ground-truth label and the predicted label (at a given threshold $\theta$), we can quantify the accuracy of the classifier on the dataset with True positives (TP($\theta$)), False positives (FP($\theta$)), False negatives (FN($\theta$)), and True negatives (TN($\theta$)). Area under the Receiver operating characteristic (ROC) curves plots two variables: True Positive Rate (TPR)
 False Positive Rate (FPR). TPR (i.e. recall) is defined as $TPR(\theta) = \frac{TP(\theta)}{TP(\theta) + FN(\theta)}$. False Positive Rate (FPR) is defined as $(\theta) = \frac{FP(\theta)}{FP(\theta) + TN(\theta)}$.

\begin{itemize}
    \item True positives, TP($\theta$), are the data points in test whose true label and predicted label equals $1$. \textit{i.e.} $y_i = 1$ and $s_i \ge \theta$
    \item False positives, FP($\theta$), are the data points in test whose true label is $0$ but the predicted label is $1$. \textit{i.e.} $y_i = 0$ and $s_i \ge \theta$.
  \item  False negatives, FN($\theta$), are data points whose true label is $1$ but the predicted label is $0$. \textit{i.e.} $y_i = 1$ and $s_i < \theta$. 
  \item True negatives, TN($\theta$), are data points whose true label is $0$ and the predicted label is $0$. \textit{i.e.} $y_i = 0$ and $s_i < \theta$. 
\end{itemize}

% We will use the notation TP($\theta$), FP($\theta$), etc. to both denote the set of corresponding data points as well as the cardinality of these sets.

The ROC curve is defined by plotting  pairs of FPR($\theta$) (x-axis) versus TPR($\theta$) (y-axis) over all possible thresholds $\theta$. ROC curve starts at $(0,0)$ and ends at $(1,1)$. The area under the ROC curve (AUC) is used to evaluate the performance of a binary classifier. If the classifier is good, the ROC curve will be close to the left and upper boundary and AUC will be close to $1.0$. On the other hand, if the classifier is poor, the ROC curve will be close to  line from $(0,0)$ to $(1,1)$ with AUC around $0.5$.

\subsection{Computing AUC with Time Complexity O(PN)}

Area under ROC curve (AUC) is well studied in statistics and is equivalent to Mann-Whitney U statistics ~\cite{AUCProb2002,dpforclassifierEvaluation}. We focus on computing the AUC by 
 viewing it as the probability of correct ranking of a random positive-negative pair. Suppose we have $M$ samples including $P$ positives and $N$ negatives, where $M = P + N$. Given a classifier $\mathcal{F}$, it gives a prediction score $s_i$ for each sample $i \in [1, M]$. We then have $MN$ positive-negative pairs with score $<s_i, s_j>$ ($i \in [1, M]$ and $j \in [1, N]$) where $s_i$ and $s_j$ are prediction scores of positive sample $i$ and negative sample $j$ respectively. Then AUC of classifier $\mathcal{F}$ is:

\begin{equation}
    \text{AUC} = \frac{I(<s_i, s_j>)}{MN}, i \in [1, M] \quad \text{and} \quad j \in [1, N]
\end{equation}

where 
\begin{equation*}
    I(<s_i, s_j>) = \begin{cases}
                    1,  \text{if} \quad s_i > s_j,\\
                    0, otherwise.
                    \end{cases}
\end{equation*}

The time complexity of computing AUC is $O(PN)$.

\subsection{Computing AUC with Time Complexity $O(M \log M)$}
\label{sec:computing_auc_ranking}

We firstly rank all instances based on their prediction scores in an increasing order. Each score $s_i$ ($i \in [1, M]$) will be assigned a ranking $r_i$. The instance with the highest order will be assigned $r = M - 1$, and the second highest one will be assigned $M -2$ and so on. The smallest ranking score is $r = 0$.

Then AUC can be computed as:

\begin{equation}
\label{eq:auc_ranking_appendix}
    \text{AUC} = \frac{\sum_{i=1}^{M} r_i \cdot y_i - \frac{P(P-1)}{2} }{PN}
\end{equation}

where $y_i \in \{0, 1\}$ is the ground-truth label for instance $i$ (with ranking score $r_i$). The time complexity of this method is $O(M\log M)$.

\section{Utility analysis of RR}
\label{sec:utility_rr}

% Then %We let the flipping probability as $r = \frac{1}{1+exp(\epsilon)}$. Then

% \begin{equation}
%     \textbf{Var}(AUC^{D_{\text{clean}}}) = \frac{\exp(\epsilon)}{(1+\exp(\epsilon))^2}\frac{M(M-1)(2M-1)/6}{P^2 * N^2}
% \end{equation}

We analyze the  variance of the computed AUC. To simplify the analysis, we use the accurate $P$ and $N$ to compute the AUC \footnote{Empirically, we did not find too much  difference between using estimated and accurate $P$ and $N$}. Let the flipping probability as $r = \frac{1}{1+exp(\epsilon)}$, then we have

% $\textbf{Var}(AUC^{D_{\text{clean}}}) = \frac{exp(\epsilon)}{(1+exp(\epsilon))^2}\frac{M(M-1)(2M-1)/6}{P^2 * N^2}$.

% We now have:

\begin{equation}
\label{eq:std_of_noisy_auc_w_accurate_p_n}
\begin{split}
\textbf{Var}(AUC^{D_{\text{clean}}})  \\ = \textbf{Var}(\frac{\sum^K sum_i - \frac{P * (P-1)}{2}}{P * N})  =  \textbf{Var}(\frac{\sum^K sum_i}{P * N}) \\= \textbf{Var}(\frac{\sum_{i=1}^P s_i (1-r)+\sum_{j=1}^N s_j r}{P * N}) \\= \frac{\sum_{i=1}^{M}s_i^2 r  (1-r)}{P^2 * N^2} = \frac{r(1-r)\sum_{i=1}^{M-1}i^2}{P^2 * N^2} \\
= r(1-r)\frac{M(M-1)(2M-1)/6}{P^2 * N^2} \\
= \frac{exp(\epsilon)}{(1+exp(\epsilon))^2}\frac{M(M-1)(2M-1)/6}{P^2 * N^2}
\end{split}
\end{equation}

%Please add the following packages if necessary:
%\usepackage{booktabs, multirow} % for borders and merged ranges
%\usepackage{soul}% for underlines
%\usepackage[table]{xcolor} % for cell colors
%\usepackage{changepage,threeparttable} % for wide tables
%If the table is too wide, replace \begin{table}[!htp]...\end{table} with
%\begin{adjustwidth}{-2.5 cm}{-2.5 cm}\centering\begin{threeparttable}[!htb]...\end{threeparttable}\end{adjustwidth}
\begin{table*}[ht!]\centering
\setlength{\tabcolsep}{0.5em} % for the horizontal padding
{% for the vertical padding
\begin{tabular}{c|c|c|c|c|c|c}\toprule
& & avg. $\#$ data samples per client &45,840 &458.4 &4.6 &1 \\ \hline
\multirow{3}{*}{$\epsilon=1.0$} &GlobalLaplace &- &4.84e-5 &5.26e-4 &4.45e-3 &1.10e-2 \\ \cline{2-7}
&\multirow{2}{*}{LocalLaplace} &i.i.d &4.81e-5 &4.66e-4 &4.25e-3 &6.44e-3 \\
& &\cellcolor[HTML]{A8A8A8}non i.i.d &\cellcolor[HTML]{A8A8A8}3.40e-5 &\cellcolor[HTML]{A8A8A8}2.98e-4 &\cellcolor[HTML]{A8A8A8}2.76e-3 &\cellcolor[HTML]{A8A8A8}6.08e-3 \\  \hline
\multirow{3}{*}{$\epsilon=2.0$} &GlobalLaplace &- &2.61e-5 &2.58e-4 &2.37e-3 &5.65e-3 \\ \cline{2-7}
&\multirow{2}{*}{LocalLaplace} &i.i.d &2.61e-5 &2.48e-4 &2.10e-3 &2.87e-3 \\
& &\cellcolor[HTML]{A8A8A8}non i.i.d &\cellcolor[HTML]{A8A8A8}1.48e-5 &\cellcolor[HTML]{A8A8A8}1.51e-4 &\cellcolor[HTML]{A8A8A8}1.38e-3 &\cellcolor[HTML]{A8A8A8}3.20e-3 \\  \hline
\multirow{3}{*}{$\epsilon=4.0$} &GlobalLaplace &- &1.30e-5 &1.21e-4 &1.21e-3 &2.68e-3 \\ \cline{2-7}
&\multirow{2}{*}{LocalLaplace} &i.i.d &1.23e-5 &1.20e-4 &1.14e-3 &1.56e-3 \\
& &\cellcolor[HTML]{A8A8A8}non i.i.d &\cellcolor[HTML]{A8A8A8}6.63e-6 &\cellcolor[HTML]{A8A8A8}7.22e-5 &\cellcolor[HTML]{A8A8A8}6.20e-4 &\cellcolor[HTML]{A8A8A8}1.69e-3 \\  \hline
\multirow{3}{*}{$\epsilon=8.0$} &GlobalLaplace &- &6.29e-6 &5.94e-5 &6.12e-4 &1.34e-3 \\ \cline{2-7}
&\multirow{2}{*}{LocalLaplace} &i.i.d &5.79e-6 &6.32e-5 &5.07e-4 &8.09e-4 \\
& &\cellcolor[HTML]{A8A8A8}non i.i.d &\cellcolor[HTML]{A8A8A8}3.98e-6 &\cellcolor[HTML]{A8A8A8}3.70e-5 &\cellcolor[HTML]{A8A8A8}3.44e-4 &\cellcolor[HTML]{A8A8A8}8.53e-4 \\
\bottomrule
\end{tabular}}
\caption{Standard deviation of estimated AUC with accurate $P$ and $N$. i.i.d: assigned samples to clients uniformly. non i.i.d: assigned samples to clients based on their prediction scores.}\label{tab:std_auc_w_accurate_P_and_N}
\end{table*}

 \section{Standard deviation of AUC with different DP budget allocation $\alpha$ in the non iid setting}
 \label{sec:std_auc_different_alpha_non_iid_appendix}

Figure ~\ref{fig:std_auc_vs_dp_allocations_non_iid_clients_1000_criteo} shows the standard deviation of AUC estimation with different allocation $\alpha$ under the Non-IID setting (1000 clients).

Figure ~\ref{fig:std_auc_vs_dp_allocations_non_iid_clients_1000_eps_4_criteo}: Standard deviation of AUC estimation with different allocation $\alpha$ under the Non-IID and IID setting with $\epsilon=4.0$ (1000 clients).
 
  \begin{figure*}[ht!]% \vspace{-0.1in}
  \centering
  \includegraphics[width=0.5\linewidth]{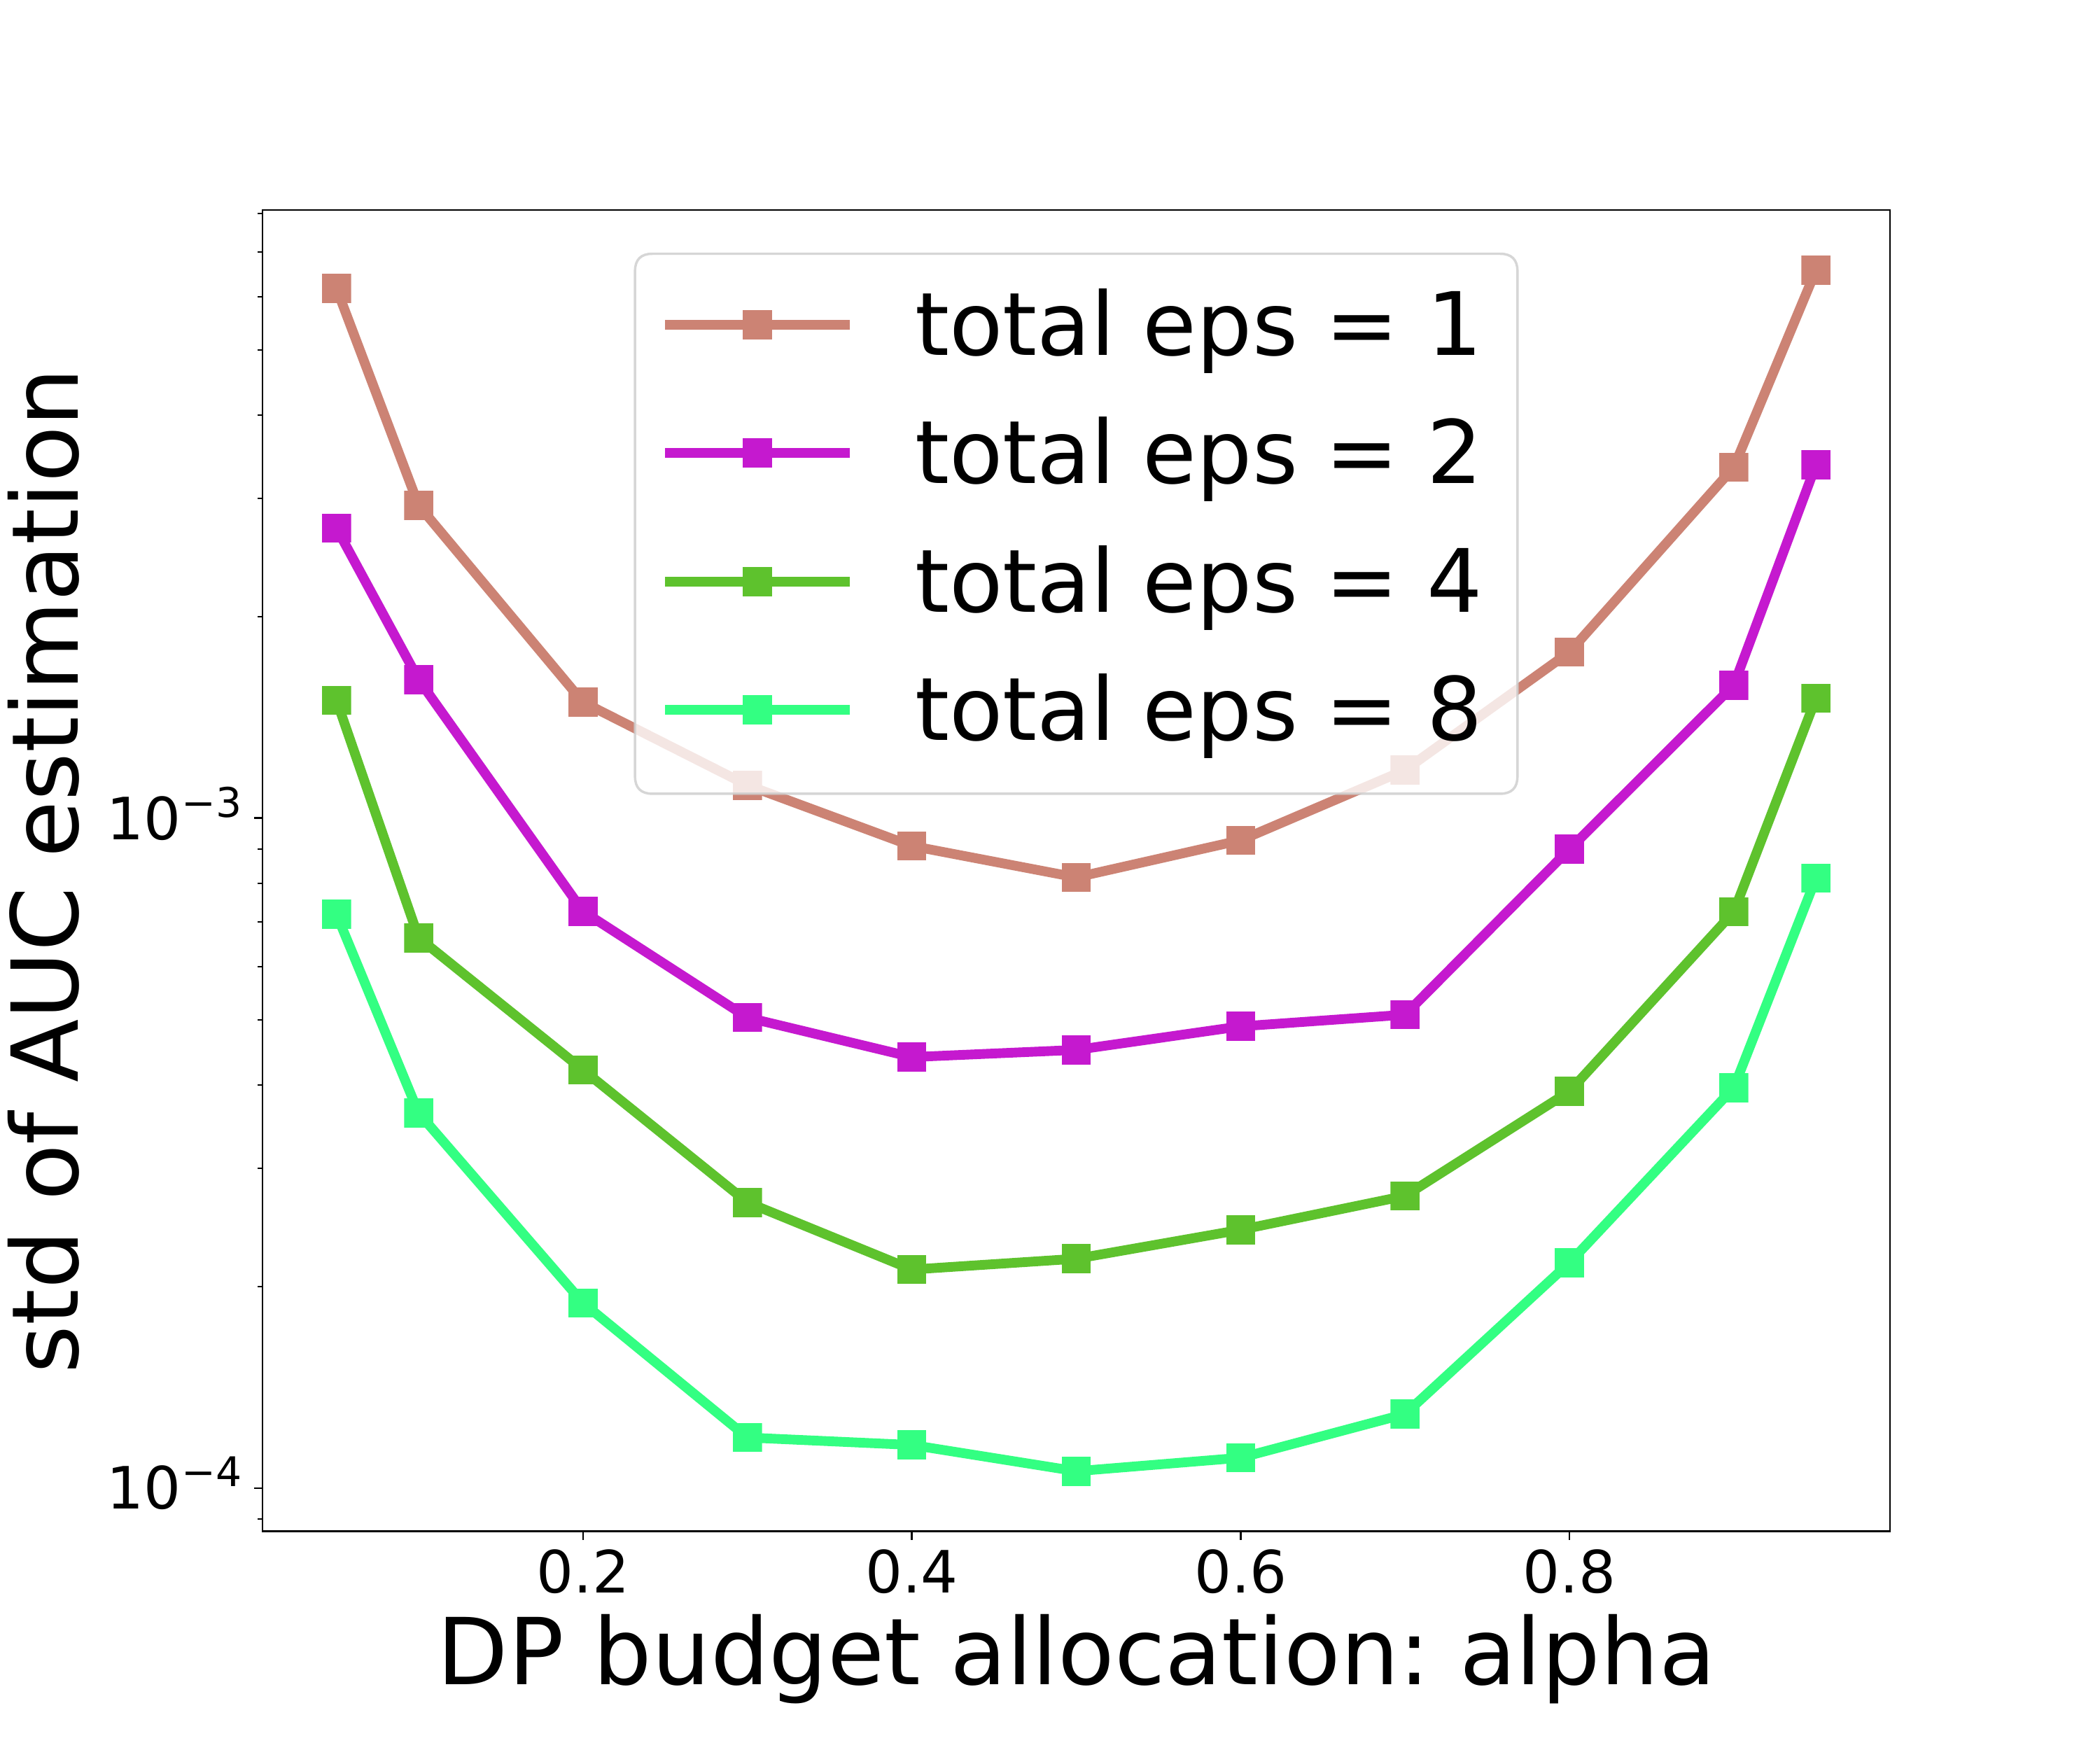}
  \caption{Standard deviation of AUC estimation with different allocation $\alpha$ under the Non-IID setting.}
 \label{fig:std_auc_vs_dp_allocations_non_iid_clients_1000_criteo} 
 \end{figure*}

 \begin{figure*}[ht!]% \vspace{-0.1in}
  \centering
  \includegraphics[width=0.5\linewidth]{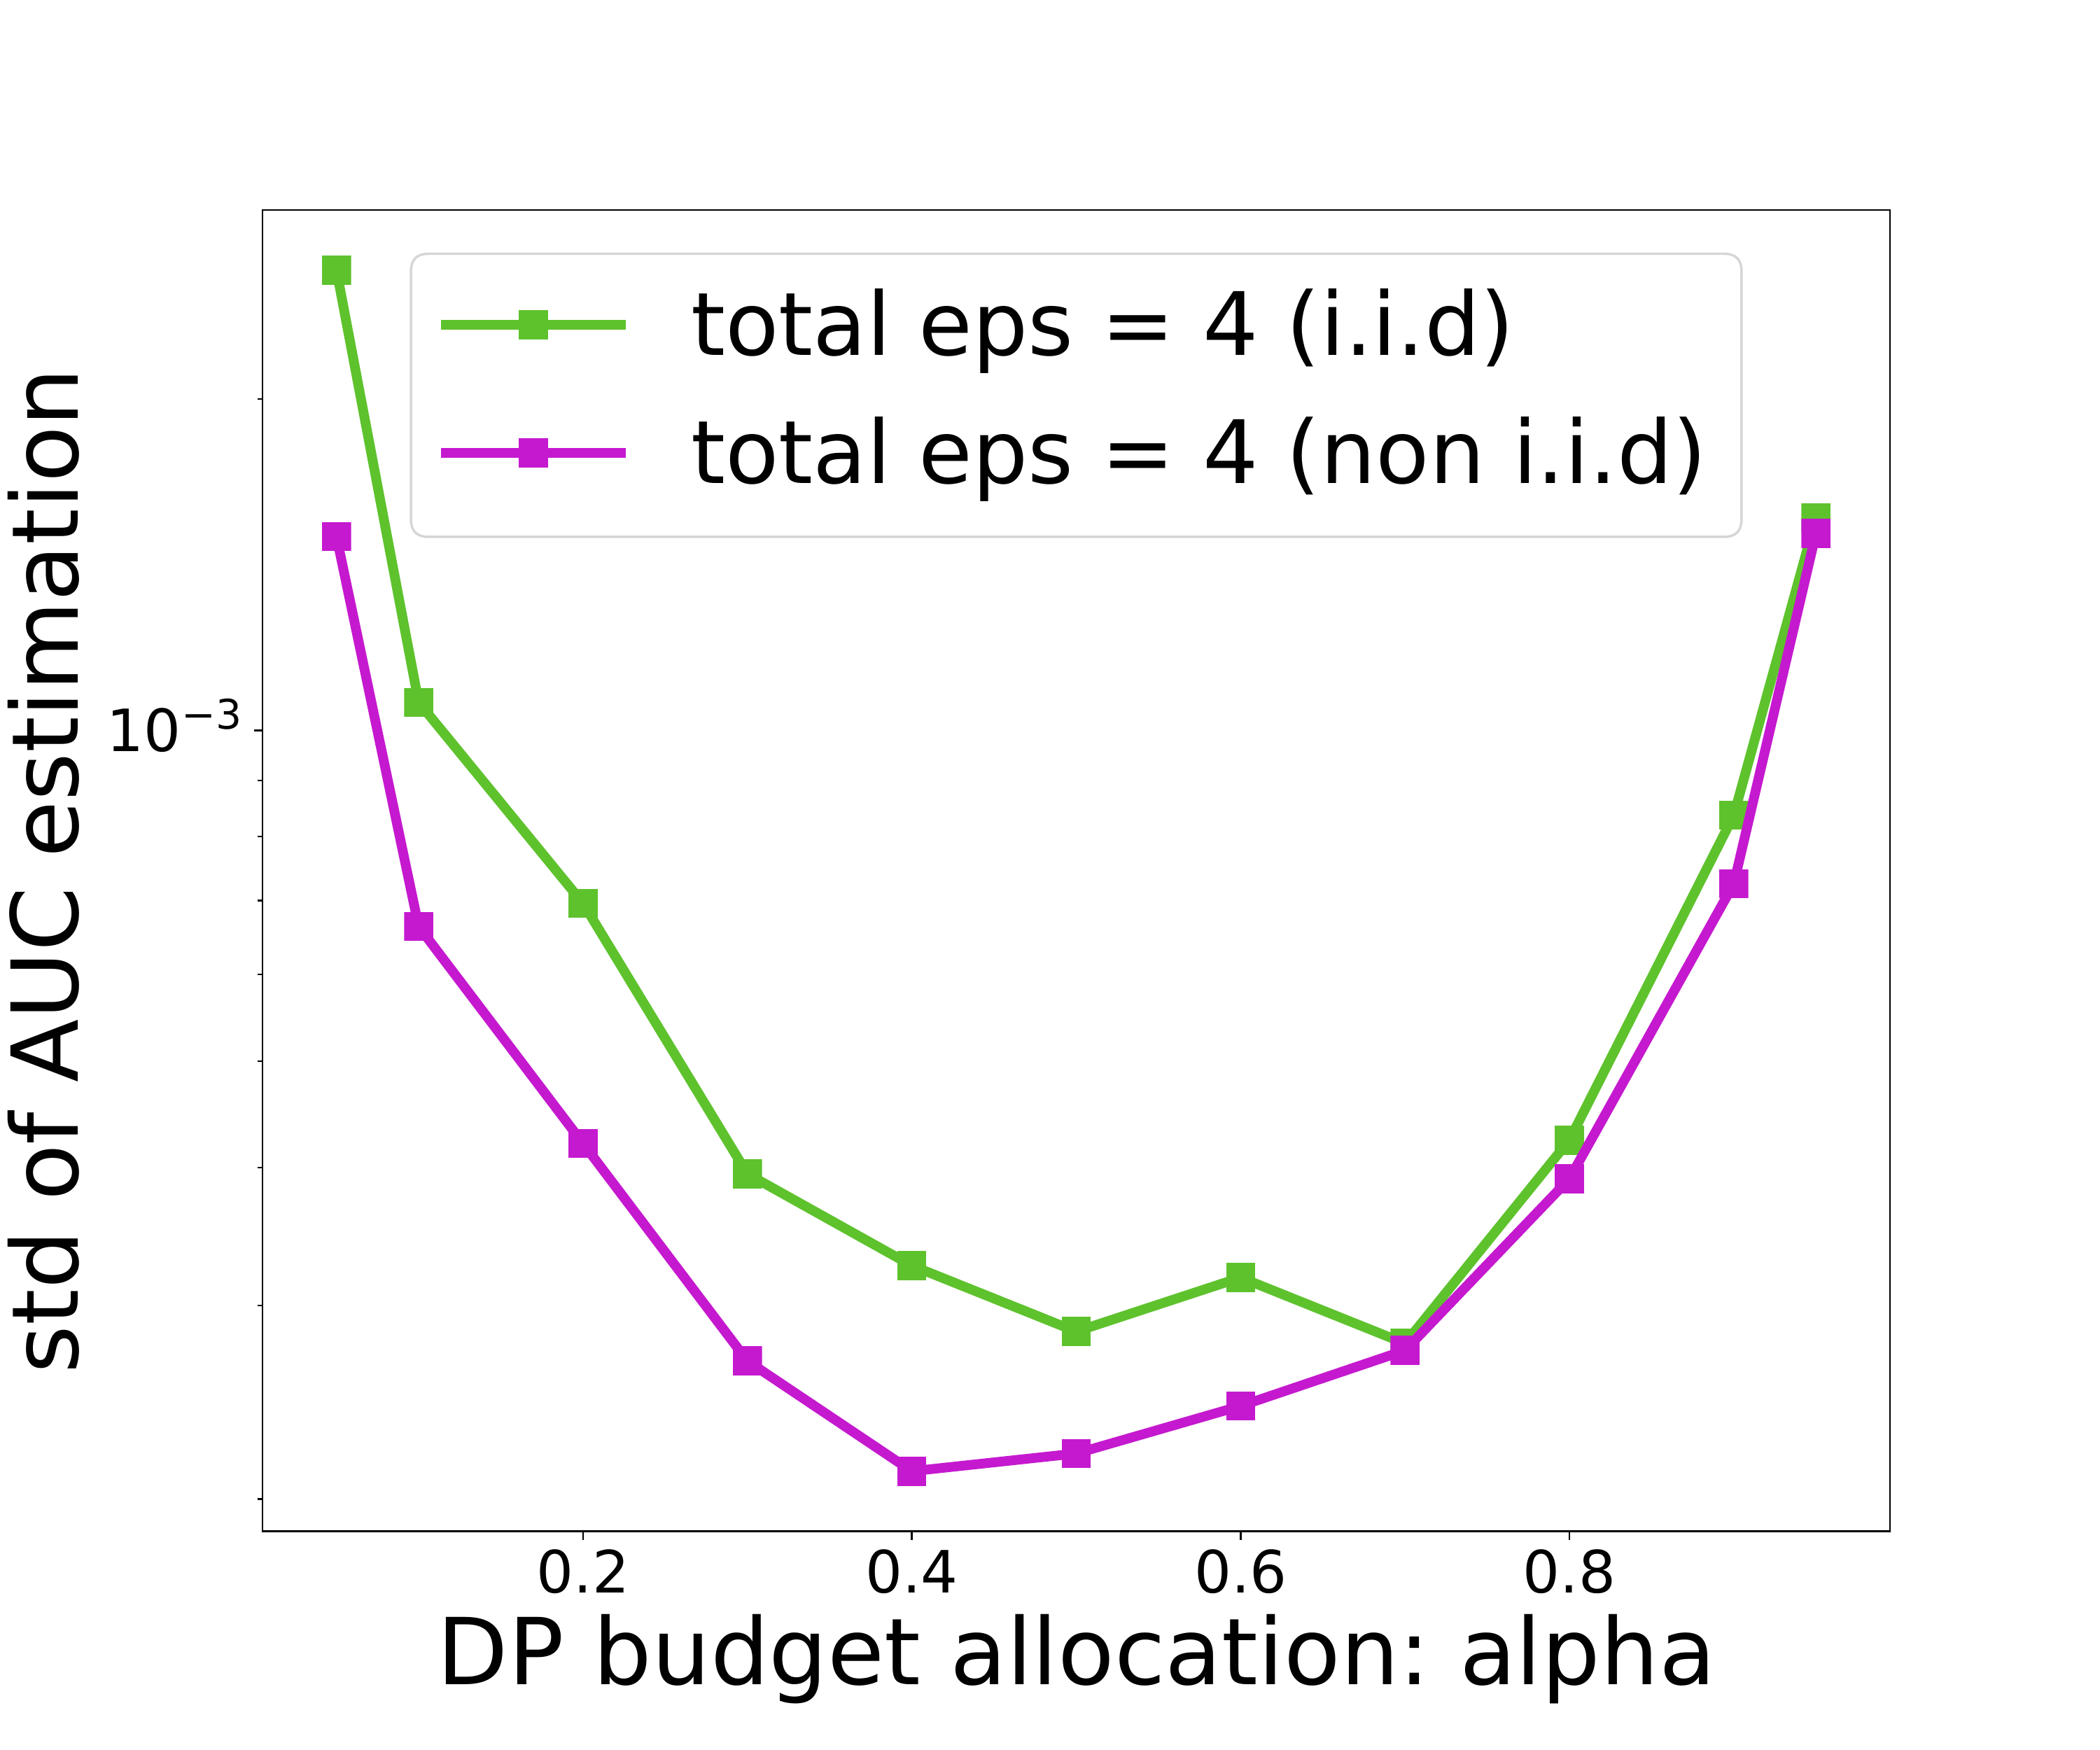}
  \caption{Standard deviation of AUC estimation with different allocation $\alpha$ under the Non-IID and IID setting with $\epsilon=4.0$.}
 \label{fig:std_auc_vs_dp_allocations_non_iid_clients_1000_eps_4_criteo} 
 \end{figure*}

 \section{Orthogonalizatin vs. Adaptive allocation in the IID setting}
 \label{sec:ortho_adaptive_iid_appendix}
 
 Figure ~\ref{fig:naive_orthogonal_adaptive_group_size_1000_eps_1} shows the std of AUC estimation with different allocation methods (Naive vs. Orthogonal vs. Adaptive) in the IID setting (1000 sampler per client) with total privacy budget $\epsilon=1$.
 
  \begin{figure*}[ht!]% \vspace{-0.1in}
  \centering
  \includegraphics[width=0.5\linewidth]{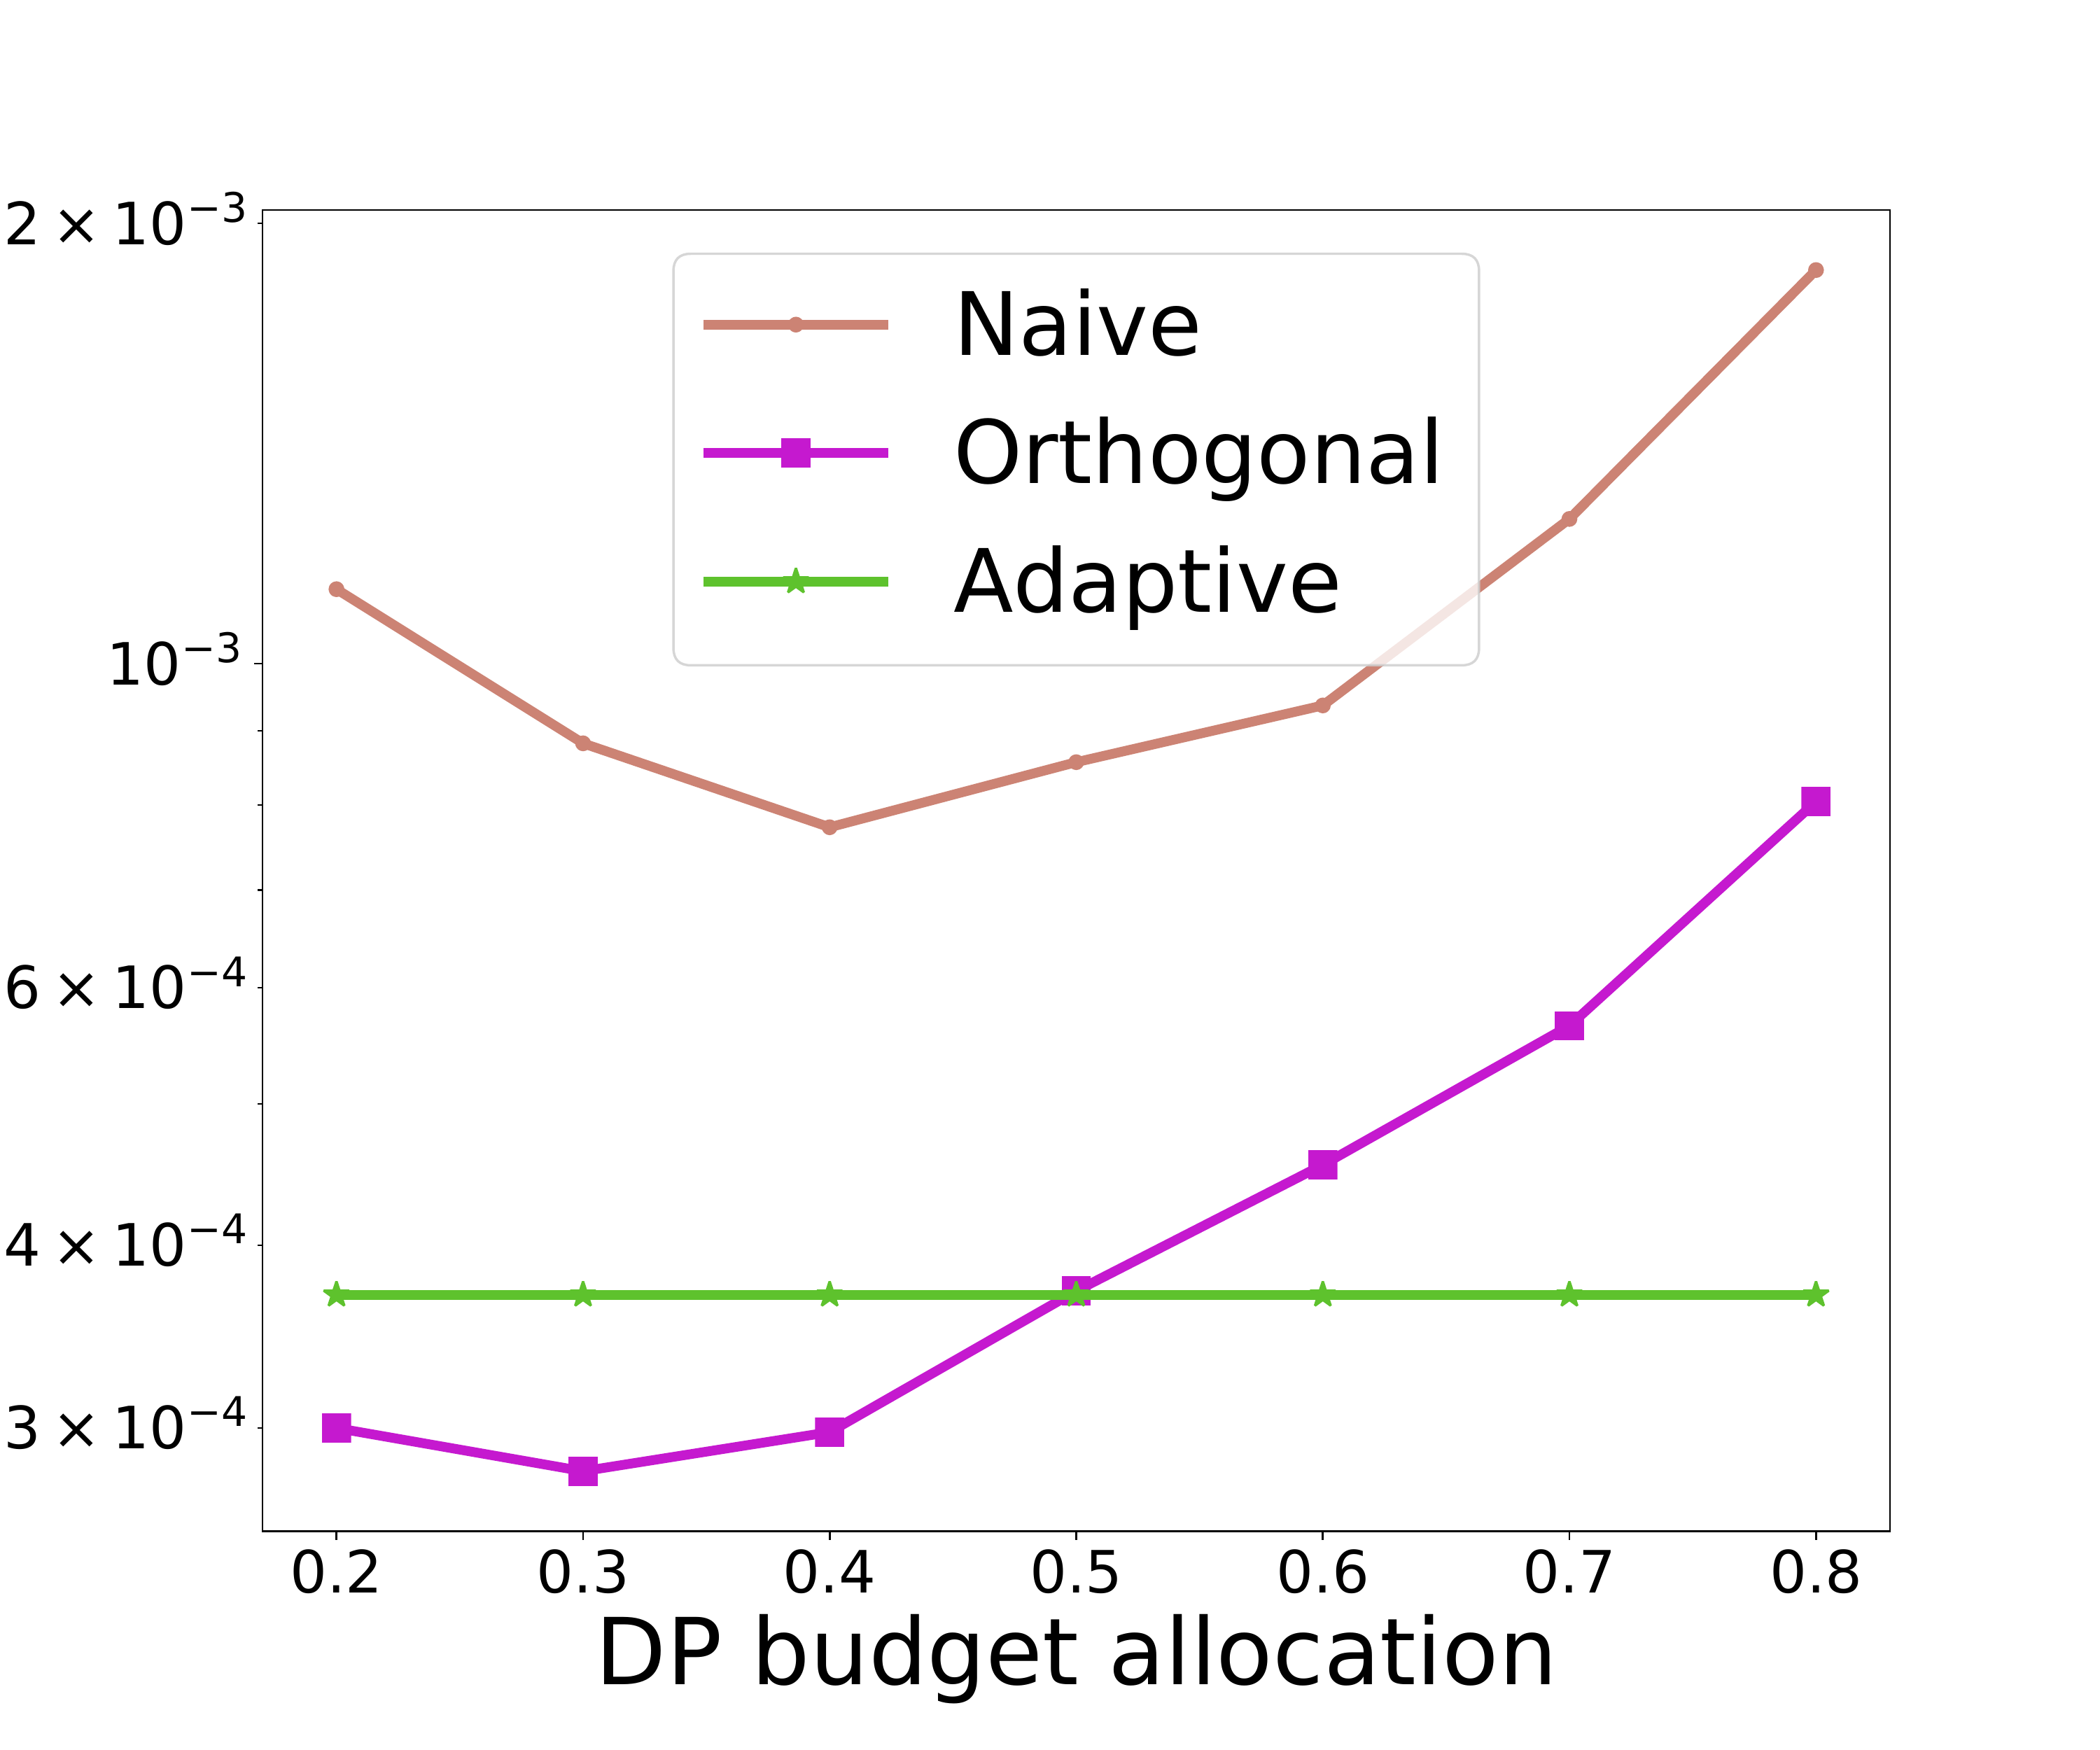}
  \caption{std of AUC estimation with different allocation methods (Naive vs. Orthogonal vs. Adaptive) in the IID setting (1000 sampler per client) with total privacy budget $\epsilon=1$.}
 \label{fig:naive_orthogonal_adaptive_group_size_1000_eps_1} 
 \end{figure*}

\section{Noisy AUC computed by Randomized Response without debiasing}
\label{sec:noisy_auc_rr_appendix}

Table ~\ref{tab:noisy_auc_randomized_response_wo_converting} shows the noisy AUC computed by randomized response only without converting it to the clean AUC (without debiasing). The utility dropping a lot with small privacy budget $\epsilon$.

%Please add the following packages if necessary:
%\usepackage{booktabs, multirow} % for borders and merged ranges
%\usepackage{soul}% for underlines
%\usepackage[table]{xcolor} % for cell colors
%\usepackage{changepage,threeparttable} % for wide tables
%If the table is too wide, replace \begin{table}[!htp]...\end{table} with
%\begin{adjustwidth}{-2.5 cm}{-2.5 cm}\centering\begin{threeparttable}[!htb]...\end{threeparttable}\end{adjustwidth}
\begin{table}[ht!]\centering
\setlength{\tabcolsep}{0.5em} % for the horizontal padding
{% for the vertical padding
\begin{tabular}{c|c|c|c|c|c}\toprule
AUC &$\epsilon$ &$\rho_{+}=\rho_{-}$ &Epoch 1 &Epoch 3 &Epoch 3 \\ \hline 
\multirow{6}{*}{Noisy AUC} &0.1 &47.50\% &0.509429 &0.510137 &0.510237 \\  \cline{2-6}
&0.5 &37.75\% &0.546986 &0.550344 &0.550862 \\ \cline{2-6}
&1 &26.89\% &0.592421 &0.598951 &0.600010 \\ \cline{2-6}
&2 &11.92\% &0.667666 &0.679436 &0.681911 \\ \cline{2-6}
&4 &1.80\% &0.735230 &0.751306 &0.754892 \\ \cline{2-6}
&10 &4.54e-5 &0.749343 &0.766438 &0.770177 \\ \hline 
scikit-learn &- &0 &0.749383 &0.766477 &0.770219 \\ \hline 
Tensorflow &- &0 &0.749382 &0.766478 &0.770219 \\
\bottomrule
\end{tabular}}
\caption{Noisy AUC computed by Randomized Response mechanism without debiasing.}\label{tab:noisy_auc_randomized_response_wo_converting}
\scriptsize
\end{table}

 \section{More results of Randomized Responses on Criteo dataset}
 \label{sec:more_results_criteo_rr_appendix}

The statistics of Criteo dataset can be seen Table ~\ref{tab:evaluation_set_statistics}. The corresponding results on small and large evaluation set can be seen in Table ~\ref{tab:auc_std_criteo} and ~\ref{tab:auc_std_criteo_large} respectively. 

 %Please add the following packages if necessary:
%\usepackage{booktabs, multirow} % for borders and merged ranges
%\usepackage{soul}% for underlines
%\usepackage[table]{xcolor} % for cell colors
%\usepackage{changepage,threeparttable} % for wide tables
%If the table is too wide, replace \begin{table}[!htp]...\end{table} with
%\begin{adjustwidth}{-2.5 cm}{-2.5 cm}\centering\begin{threeparttable}[!htb]...\end{threeparttable}\end{adjustwidth}
\begin{table*}[ht!]\centering
\setlength{\tabcolsep}{0.5em} % for the horizontal padding
{% for the vertical padding
\begin{tabular}{|c|c|c|c|c|}\toprule
& $\#$ Positives ($P$) & $\#$ Negatives ($N$) & $\#$ Total ($M$) \\ \hline
Small Criteo Evaluation Set &117,317 &341,090 &458,407 \\ \hline
Large Criteo Evaluation Set &1,173,981 &3,410,081 &4,584,062 \\ 
\bottomrule
\end{tabular}}
\caption{Statistics of Two Criteo Evaluation Sets}\label{tab:evaluation_set_statistics}
\end{table*}
 
%Please add the following packages if necessary:
%\usepackage{booktabs, multirow} % for borders and merged ranges
%\usepackage{soul}% for underlines
%\usepackage[table]{xcolor} % for cell colors
%\usepackage{changepage,threeparttable} % for wide tables
%If the table is too wide, replace \begin{table}[!htp]...\end{table} with
%\begin{adjustwidth}{-2.5 cm}{-2.5 cm}\centering\begin{threeparttable}[!htb]...\end{threeparttable}\end{adjustwidth}
\begin{table*}[ht!]\centering
% \scriptsize
\setlength{\tabcolsep}{0.5em} % for the horizontal padding
{% for the vertical padding
\begin{tabular}{|c|c|c|c|c|c|c}\toprule
AUC and std &$\epsilon$ &$\rho_{+}=\rho_{-}$ &Epoch 1 &Epoch 2 &Epoch 3 \\ \hline
\multirow{10}{*}{\ourapprr{}} &0.1 &47.50\% &0.745667 $\pm$ 2.41$\text{e-}$2 &0.765312 $\pm$ 2.40$\text{e-}$2 &0.777627 $\pm$ 2.62$\text{e-}$2 \\ \cline{2-6}
&0.25 &43.78\% &0.749169 $\pm$ 8.69$\text{e-}$3 &0.767502 $\pm$ 8.76$\text{e-}$3 &0.771198 $\pm$ 7.57$\text{e-}$3 \\ \cline{2-6}
&0.5 &37.75\% &0.749206 $\pm$ 5.39$\text{e-}$3 &0.767081 $\pm$ 4.79$\text{e-}$3 &0.769621 $\pm$ 4.56$\text{e-}$3 \\ \cline{2-6}
&1 &26.89\% &0.749495 $\pm$ 2.11$\text{e-}$3 &0.766833 $\pm$ 2.09$\text{e-}$3 &0.770707 $\pm$ 2.23$\text{e-}$3 \\ \cline{2-6}
&2 &11.92\% &0.749453 $\pm$ 9.43$\text{e-}$4 &0.766621 $\pm$ 8.76$\text{e-}$4 &0.770548 $\pm$ 1.01$\text{e-}$3 \\ \cline{2-6}
&3 &4.74\% &0.749295 $\pm$ 5.46$\text{e-}$4 &0.766490 $\pm$ 4.62$\text{e-}$4 &0.770183 $\pm$ 6.14$\text{e-}$4 \\ \cline{2-6}
&4 &1.80\% &0.749207 $\pm$ 3.75$\text{e-}$4 &0.766458 $\pm$ 3.33$\text{e-}$4 &0.770161 $\pm$ 3.21$\text{e-}$4 \\ \cline{2-6}
&5 &0.67\% &0.749399 $\pm$ 2.05$\text{e-}$4 &0.766477 $\pm$ 2.14$\text{e-}$4 &0.770214 $\pm$ 1.33$\text{e-}$4 \\ \cline{2-6}
&10 &4.54$\text{e-}$5 &0.749383 $\pm$ 1.77$\text{e-}$5 &0.766475 $\pm$ 1.84$\text{e-}$5 &0.770214 $\pm$ 1.67$\text{e-}$5 \\ \cline{2-6}
&$+ \infty$ &0 &0.749383 $\pm$ 0.00$\text{e+}$0 &0.766477 $\pm$ 0.00$\text{e+}$0 &0.770219 $\pm$ 0.00$\text{e+}$0 \\ \hline
scikit-learn &- &0 &0.749383  $\pm$ 1.11$\text{e-}$16  &0.766477 $\pm$ 1.11$\text{e-}$16 &0.770219 $\pm$ 1.11$\text{e-}$16 \\ \hline
Tensorflow &- &0 &0.749382 $\pm$ 5.96$\text{e-}$8 &0.766478 $\pm$ 5.96$\text{e-}$8 &0.770219 $\pm$ 5.96$\text{e-}$8 \\
\hline
\end{tabular}} 
\caption{Mean and standard deviation (std) of AUC computed by \ourapprr{} and ground-truth on the Criteo evaluation set. }
\label{tab:auc_std_criteo}
\end{table*}

%Please add the following packages if necessary:
%\usepackage{booktabs, multirow} % for borders and merged ranges
%\usepackage{soul}% for underlines
%\usepackage[table]{xcolor} % for cell colors
%\usepackage{changepage,threeparttable} % for wide tables
%If the table is too wide, replace \begin{table}[!htp]...\end{table} with
%\begin{adjustwidth}{-2.5 cm}{-2.5 cm}\centering\begin{threeparttable}[!htb]...\end{threeparttable}\end{adjustwidth}
\begin{table*}[ht!]\centering
\setlength{\tabcolsep}{0.5em} % for the horizontal padding
{% for the vertical padding
\begin{tabular}{|c|c|c|c|c|c|c|}\toprule
&$\epsilon$ &$\rho_{+}=\rho_{-}$ &Epoch 1 &Epoch 2 &Epoch 3 \\ \hline
\multirow{10}{*}{\ourapprr{}} &0.1 &47.50\% &0.751439\ $\pm$ 7.52$\text{e-}$3 &0.768640\ $\pm$ 6.96$\text{e-}$3 &0.774664\ $\pm$ 6.48$\text{e-}$3 \\ \cline{2-6}
&0.25 &43.78\% &0.750405\ $\pm$ 2.90$\text{e-}$3 &0.767958\ $\pm$ 2.85$\text{e-}$3 &0.771694\ $\pm$ 3.26$\text{e-}$3 \\ \cline{2-6}
&0.5 &37.75\% &0.750589\ $\pm$ 1.32$\text{e-}$3 &0.768324\ $\pm$ 1.62$\text{e-}$3 &0.772143\ $\pm$ 1.39$\text{e-}$3 \\ \cline{2-6}
&1 &26.89\% &0.750345\ $\pm$ 5.51$\text{e-}$4 &0.767988\ $\pm$ 7.27$\text{e-}$4 &0.771974\ $\pm$ 8.11$\text{e-}$4 \\ \cline{2-6}
&2 &11.92\% &0.750482\ $\pm$ 3.03$\text{e-}$4 &0.768001\ $\pm$ 3.03$\text{e-}$4 &0.772005\ $\pm$ 3.60$\text{e-}$4 \\ \cline{2-6}
&3 &4.74\% &0.750480\ $\pm$ 1.53$\text{e-}$4 &0.768043\ $\pm$ 1.82$\text{e-}$4 &0.772040\ $\pm$ 1.73$\text{e-}$4 \\ \cline{2-6}
&4 &1.80\% &0.750509\ $\pm$ 9.45$\text{e-}$5 &0.768055\ $\pm$ 1.11$\text{e-}$4 &0.772008\ $\pm$ 1.20$\text{e-}$4 \\ \cline{2-6}
&5 &0.67\% &0.750500\ $\pm$ 5.87$\text{e-}$5 &0.768041\ $\pm$ 6.73$\text{e-}$5 &0.772004\ $\pm$ 6.11$\text{e-}$5 \\ \cline{2-6}
&10 &4.54e-5 &0.750509\ $\pm$ 5.37$\text{e-}$6 &0.768046\ $\pm$ 5.83$\text{e-}$6 &0.772008\ $\pm$ 5.04$\text{e-}$6 \\ \cline{2-6}
&$+\infty$ &0 &0.750509\ $\pm$ 0.00$\text{e+}$0 &0.768045\ $\pm$ 1.11$\text{e-}$16 &0.772007\ $\pm$ 1.11$\text{e-}$16 \\ \hline
scikit-learn &- &0 &0.750509\ $\pm$ 1.11$\text{e-}$16 &0.768045\ $\pm$ 1.11$\text{e-}$16 &0.772007\ $\pm$ 1.11$\text{e-}$16 \\ \hline
Tensorflow &- &0 &0.750509\ $\pm$ 5.96$\text{e-}$8 &0.768044\ $\pm$ 5.96$\text{e-}$8 &0.772006\ $\pm$ 5.96$\text{e-}$8 \\
\bottomrule
\end{tabular}}
\caption{Mean and standard deviation (std) of AUC computed by FedAUC and baselines on large Criteo evaluation set.}\label{tab:auc_std_criteo_large}
\end{table*}

\section{Variance of AUC estimated by GlobalLaplace}
\label{sec:var_auc_globallaplace}

We also add a comparison partner \globallap{} here. All clients use $M - 1$ as the sensitivity when adding noise to their local statistics $\text{localSum}$. Given a privacy budget $\epsilon_{localSum}$, client $C_k$ draws the random noise from $Lap((M-1)/\epsilon_{localSum})$. Each client will add the same amount of noise to its $\text{localSum}$. Given $P$ and $N$ are accurate, the corresponding standard deviation of computed AUC is $std(AUC_{\text{\globallap{}}}) = \frac{\sqrt{2K}(M-1)}{P* N * \epsilon}$. Since
 
 \begin{equation}
 \label{eq:var_globallap}
 \textbf{Var}(AUC_{\text{\globallap{}}})   = \textbf{Var}(\frac{\sum^K sum_i - \frac{P * (P-1)}{2}}{P * N})  =  \textbf{Var}(\frac{\sum^K sum_i}{P * N}) = \frac{K * \sigma^2}{P^2 * N^2} = \frac{2K(M-1)^2}{P^2 * N^2 * \epsilon^2}
 \end{equation}

 \section{Utility analysis of LocalLaplace}
\label{sec:utility_analysis_locallap_appendix}

To simplify the analysis, we assume that $P$ and $N$ are accurate\footnote{only adding noise to $\text{localSum}$} and each client only has one data sample\footnote{$\text{sum}_i \in [1, K-1]$}, the standard deviation of computed AUC by \locallap{} is:

\begin{equation}
\label{eq:var_locallap}
   \textbf{Var} (\text{AUC}_{\text{\locallap{}}})  =  \textbf{Var}(\frac{\sum_{i=1}^K sum_i}{P  N}) =  \frac{\sum_{i=1}^{K-1} 2*i^2 / \epsilon^2}{P^2  N^2} = \frac{K(K-1)(2K-1)}{3P^2  N^2  \epsilon^2}
\end{equation} 
 
 \section{Estimate $\pi'$}
 \label{sec:estimate_pi}
 
 Suppose we observe $\bar{M}$ positive examples and $\bar{N}$ negative examples in the corrupted data $D'$. We have:

\begin{equation}
    P'+N' = \bar{P}+\bar{N}, \quad P'(1-\rho_{+}) + N \rho_{-} = \bar{P}
\end{equation}

where $P'$ and $N'$ are estimated positive and negative numbers in the clean data $D$.

We then obtain:

\begin{equation}
    P' = \frac{\bar{P}(1-\rho_{-}) - \bar{N}\rho_{-}}{1-\rho_{+}-\rho_{-}}, \quad N'= \bar{P}+\bar{N}-P'
\end{equation}

Then we use $P'$ and $N'$ to  estimate  base rate $\pi$ as $\pi'$:

\begin{equation}
    \pi' = \frac{P'}{P' + N'}
\end{equation}

\section{Table ~\ref{tab:std_auc_w_noisy_P_and_N}: std of AUC estimated different methods: RR vs. GlobalLaplace vs. LocalLapace with Adaptive Budget Allocation}
\label{sec:compare_all_methods_auc_appendix}

Table ~\ref{tab:std_auc_w_noisy_P_and_N} shows the std of AUC estimated by different methods (RR vs. GlobalLaplace vs. LocalLapace with Adaptive Budget Allocation).

\begin{table}[!htp]\centering
\scriptsize 
\setlength{\tabcolsep}{0.5em} % for the horizontal padding
{% for the vertical padding
\begin{tabular}{c|c|c|c|c|c|c|c|c}\toprule
&$\#$ clients &10 &458 &1,000 &4,584 &45,840 &100,000 &458,407 \\ \hline 
&avg. $\#$ data samples per client &45,840.00 &1,000.00 &458.40 &100.00 &10.00 &4.60 &1 \\ \hline 
\multirow{4}{*}{$\epsilon=1.0$} &RR &\multicolumn{7}{c}{2.17e-3} \\ \cline{2-9}
&GlobalLaplace &1.22e-4 &8.48e-4 &1.24e-3 &2.39e-3 &8.08e-3 &1.24e-2 &2.77e-2 \\ \cline{2-9}
&LocalLaplace (IID) &1.13e-4 &9.64e-4 &1.26e-3 &2.26e-3 &7.39e-3 &1.10e-2 &1.99e-2 \\ \cline{2-9}
&\cellcolor[HTML]{A8A8A8}LocalLaplace (Non-IID) &\cellcolor[HTML]{A8A8A8}8.98e-5 &\cellcolor[HTML]{A8A8A8}5.29e-4 &\cellcolor[HTML]{A8A8A8}8.49e-4 &\cellcolor[HTML]{A8A8A8}1.86e-3 &\cellcolor[HTML]{A8A8A8}5.45e-3 &\cellcolor[HTML]{A8A8A8}8.33e-3 &\cellcolor[HTML]{A8A8A8}1.81e-2 \\ 
&adaptive (IID) &5.15e-5 &3.92e-4 & & 1.22e-3& 3.80e-3& & \\ \cline{2-9}
&adaptive (non-IID) &2.93e-5 &1.22e-4 & & 3.92e-4& 1.03e-3& & \\ \cline{2-9}
\hline 
\multirow{4}{*}{$\epsilon=2.0$} &RR &\multicolumn{7}{c}{1.02e-3} \\ \cline{2-9} 
&GlobalLaplace &5.85e-5 &4.15e-4 &5.62e-4 &1.28e-3 &3.95e-3 &5.21e-3 &1.32e-2 \\ \cline{2-9} 
&LocalLaplace (IID) &5.74e-5 &4.72e-4 &5.78e-4 &1.21e-3 &4.09e-3 &5.24e-3 &8.86e-3 \\ \cline{2-9}
&\cellcolor[HTML]{A8A8A8}LocalLaplace (Non-IID) &\cellcolor[HTML]{A8A8A8}4.59e-5 &\cellcolor[HTML]{A8A8A8}2.91e-4 &\cellcolor[HTML]{A8A8A8}4.93e-4 &\cellcolor[HTML]{A8A8A8}9.45e-4 &\cellcolor[HTML]{A8A8A8}3.09e-3 &\cellcolor[HTML]{A8A8A8}4.38e-3 &\cellcolor[HTML]{A8A8A8}9.96e-3 \\ 
&adaptive (IID) & 2.60e-5&1.84e-4 & & 6.48e-4& 1.66e-3& & \\ \cline{2-9}
&adaptive (non-IID) & 1.59e-5&6.01e-5 & & 1.52e-4& 5.54e-4& & \\ \cline{2-9}
\hline 
\multirow{4}{*}{$\epsilon=4.0$} &RR &\multicolumn{7}{c}{3.49e-4} \\ \cline{2-9} 
&GlobalLaplace &2.92e-5 &2.09e-4 &3.26e-4 &6.58e-4 &1.88e-3 &3.22e-3 &7.02e-3 \\ \cline{2-9} 
&LocalLaplace (IID) &3.11e-5 &1.94e-4 &3.00e-4 &5.80e-4 &1.86e-3 &2.40e-3 &4.38e-3 \\ \cline{2-9}
&\cellcolor[HTML]{A8A8A8}LocalLaplace (Non-IID) &\cellcolor[HTML]{A8A8A8}2.49e-5 &\cellcolor[HTML]{A8A8A8}1.48e-4 &\cellcolor[HTML]{A8A8A8}2.05e-4 &\cellcolor[HTML]{A8A8A8}4.44e-4 &\cellcolor[HTML]{A8A8A8}1.53e-3 &\cellcolor[HTML]{A8A8A8}2.26e-3 &\cellcolor[HTML]{A8A8A8}4.39e-3 \\ 
&adaptive (IID) & 1.36e-5&8.20e-5 & & 2.87e-4& 9.08e-4& & \\ \cline{2-9}
&adaptive (non-IID) & 7.80e-6&2.81e-5 & & 8.72e-5& 2.77e-4& & \\ \cline{2-9}
\hline 
\multirow{4}{*}{$\epsilon=8.0$} &RR &\multicolumn{7}{c}{4.41e-5} \\ \cline{2-9}
&GlobalLaplace &1.54e-5 &9.82e-5 &1.53e-4 &3.31e-4 &1.05e-3 &1.58e-3 &2.99e-3 \\\cline{2-9}
&LocalLaplace (IID) &1.51e-5 &1.06e-4 &1.40e-4 &3.27e-4 &8.52e-4 &1.35e-3 &2.29e-3 \\\cline{2-9}
&\cellcolor[HTML]{A8A8A8}LocalLaplace (Non-IID) &\cellcolor[HTML]{A8A8A8}1.06e-5 &\cellcolor[HTML]{A8A8A8}6.99e-5 &\cellcolor[HTML]{A8A8A8}1.14e-4 &\cellcolor[HTML]{A8A8A8}2.19e-4 &\cellcolor[HTML]{A8A8A8}7.50e-4 &\cellcolor[HTML]{A8A8A8}1.16e-3 &\cellcolor[HTML]{A8A8A8}2.22e-3 \\
&adaptive (IID) &7.01e-6 &4.55e-5 & & 1.37e-4& 4.61e-4& & \\ \cline{2-9}
&adaptive (non-IID) &3.89e-6 &1.36e-5 & & 4.34e-5& 1.38e-4& & \\ \cline{2-9}
\hline 
\bottomrule
\end{tabular}}
\caption{Standard deviation of AUC estimated by different methods (DP budget allocation $\alpha = 0.5$ which means that $\epsilon_{\text{localSum}} = \epsilon_{\text{localP}} = 0.5\epsilon$). IID: assigned samples to clients uniformly. Non-IID: assigned samples to clients based on their prediction scores.}\label{tab:std_auc_w_noisy_P_and_N}
\end{table}

\section{Privacy Analysis of Prediction Scores}
\label{sec:sorting_module} 

In this section, we talk about how clients know the ranking results of their prediction scores and the corresponding privacy issue. 

In the vanilla setting, each client $C_k$ can send its shuffled prediction scores $s^k$ to the server. The server then aggregates all the prediction scores and sort them in an increasing order. Each prediction score $s_i^k$ ($i \in [1, M]$) will be assigned a ranking order $r_i^k$. The instance with the highest order will be assigned $r = M - 1$, and the second highest one will be assigned $M -2$ and so on. The smallest ranking score is $r = 0$. The server sends each ranking order $r_i^k$ back to the corresponding client $C_k$ which owns $s_i^k$. 
It's worth mentioning the prediction scores have to be shared with the server for some tasks. For example, the clients have to report the predicted conversion rate (CVR) of the ad impression to the server in online advertisements. The server \footnote{ad exchange} can later on calculate the bid price by multiplying the predicted CVR with  a constant parameter tuned according to the campaign budget and performance ~\cite{bidding2018}. Then the server can select the advertiser who proposed the highest bid price as the winner to show the ad.

\input{tables/top_k_analysis_criteo_data}

 \begin{figure}[ht!]% \vspace{-0.1in}
  \centering
    \includegraphics[width=0.75\linewidth]{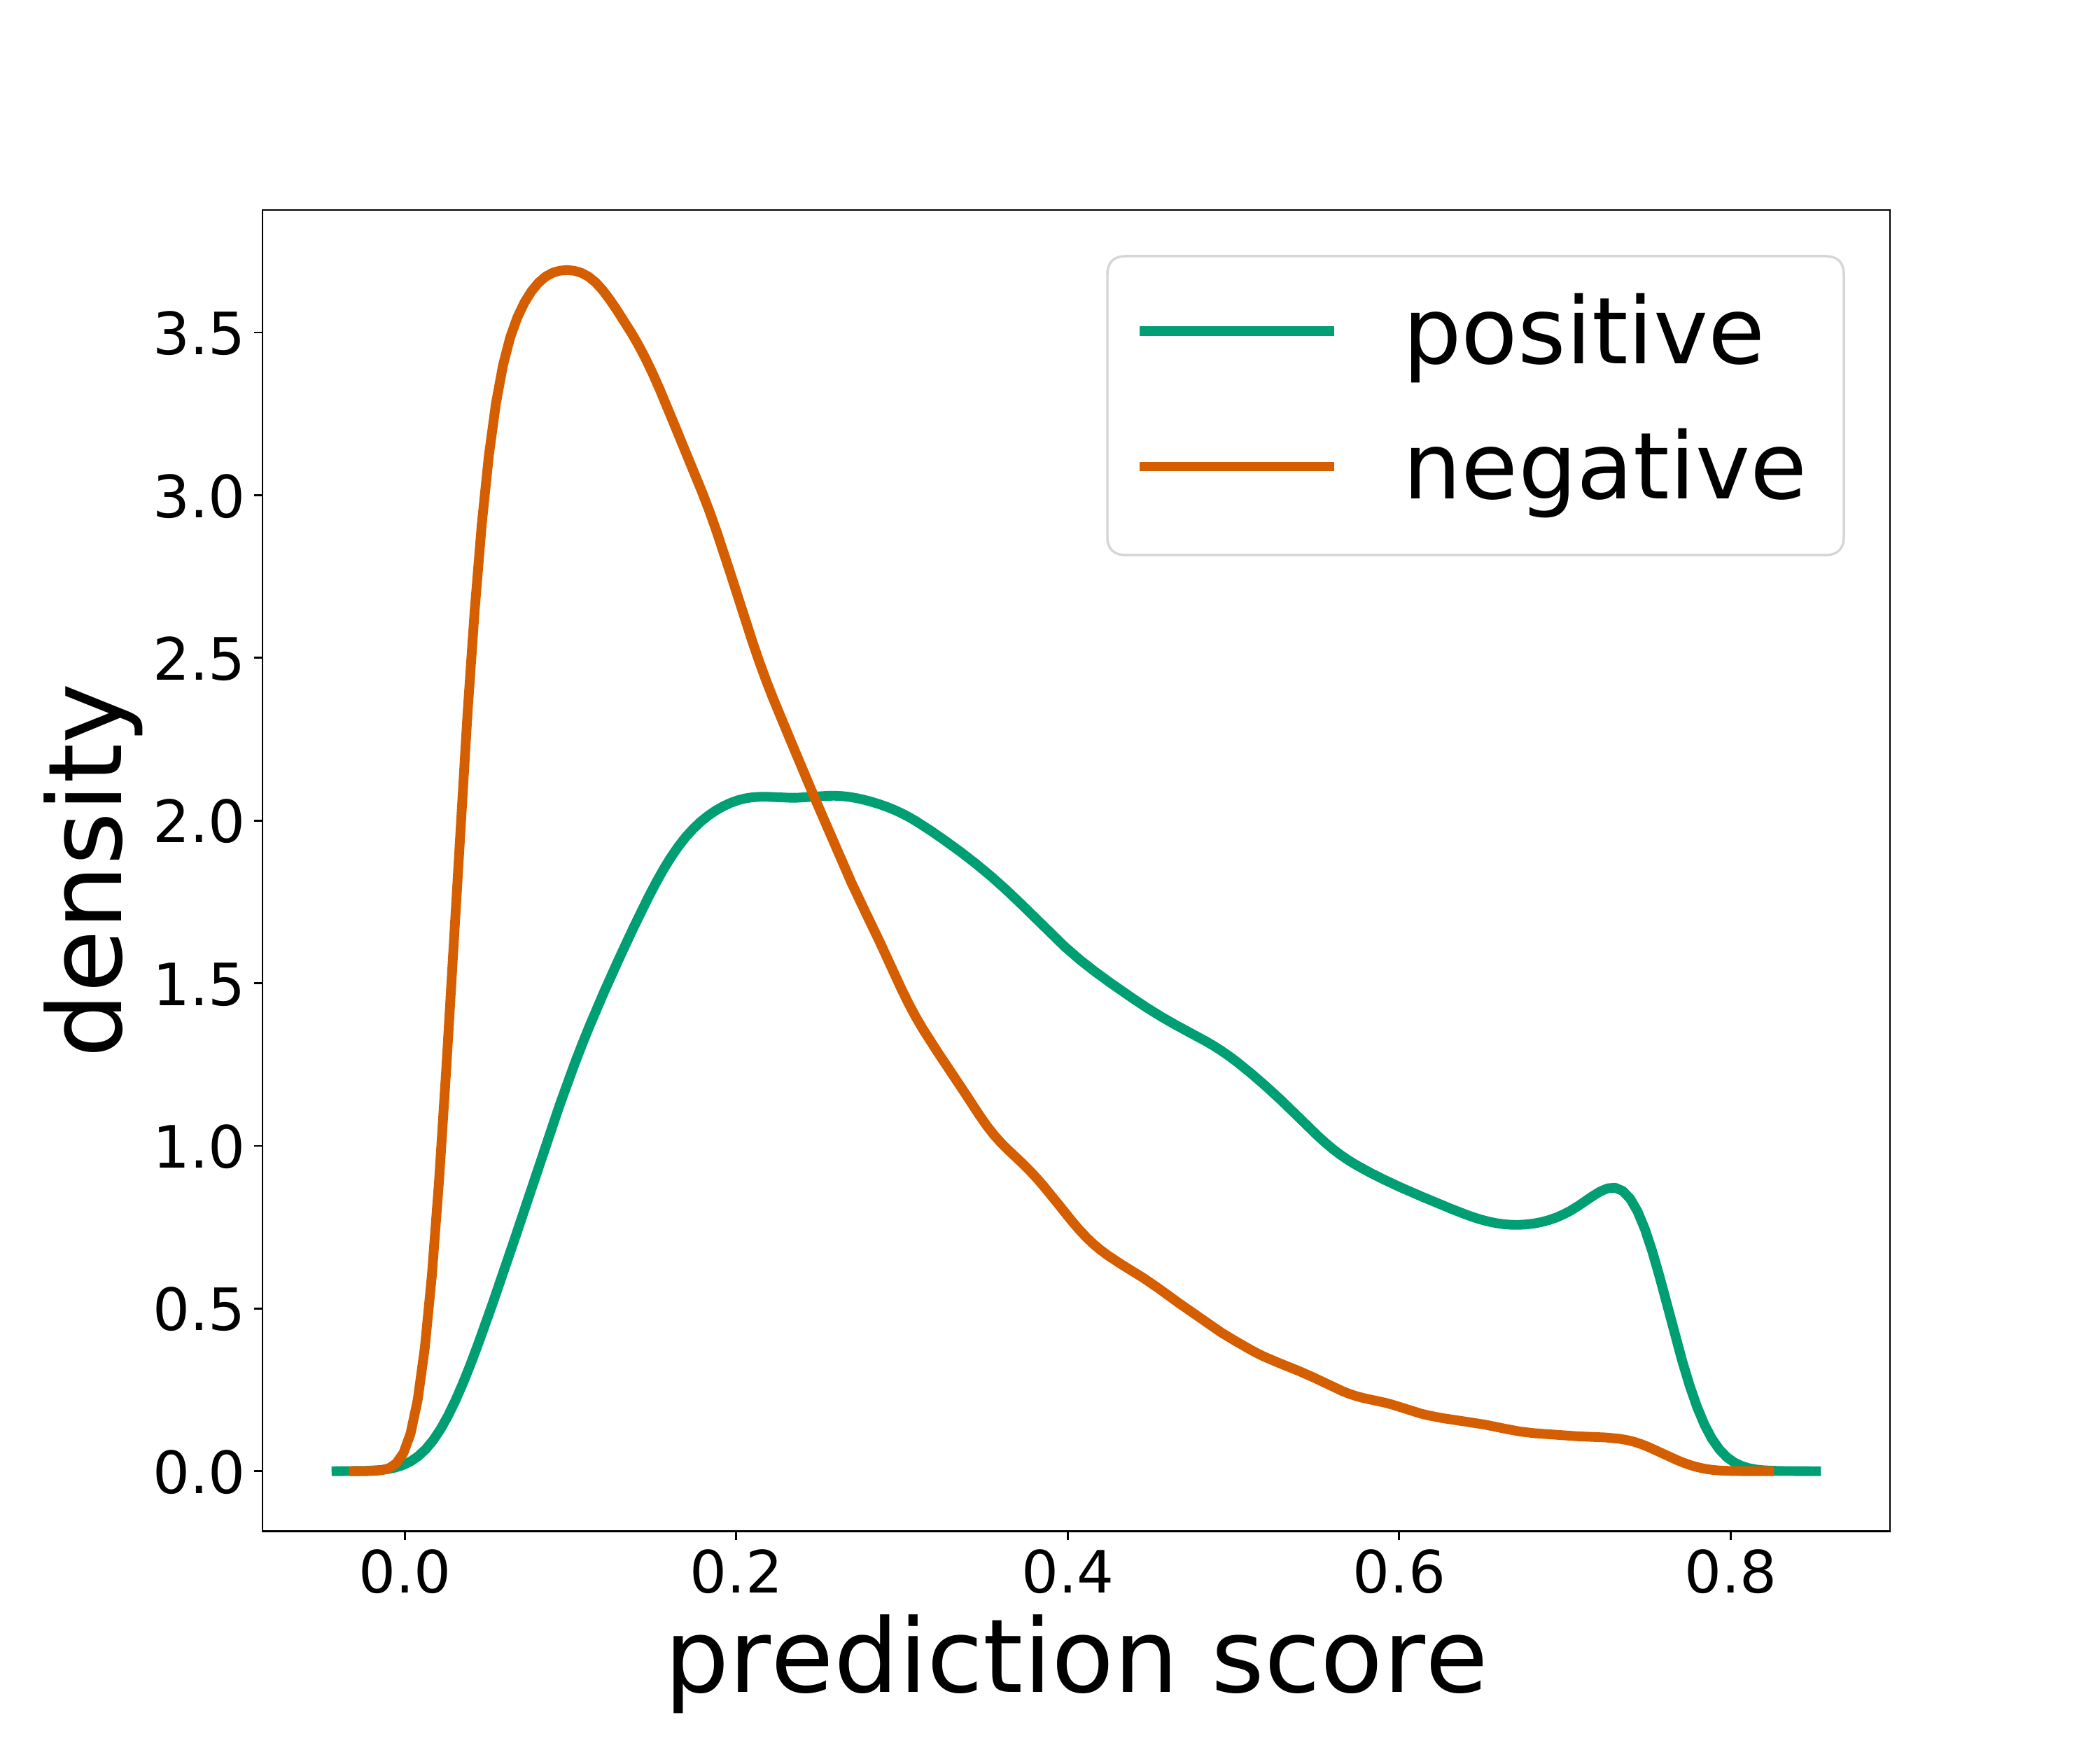}
  \caption{Density of positive and negative instances' prediction scores in Criteo data.}
 \label{fig:criteo_negative_positive_density} 
 \end{figure}

Interested readers may be curious if is it possible to infer the label information based on the prediction scores. Here we propose a simple attack method by selecting the samples with top-K prediction scores as positive labels. We measure the corresponding guessing performance by precision and recall. As shown in Figure ~\ref{fig:criteo_negative_positive_density} and Table ~\ref{tab:top_k_analysis_criteo_data_small}, positive instances can have a relative higher prediction scores than negative ones at some density areas. For example, we can achieve a $79\%$ precision if we select the instances with top-$100$ prediction scores. However, since the prediction scores $s^k$ are shuffled before sending to the server so that the server has no idea which prediction score belongs to which data sample \footnote{$|s^k| \geq 2$}. 

Instead of the vanilla setting, we also propose some alternative solutions to achieve the sorting goal. We may leverage DP to add noise to the prediction scores. Since the prediction score is the output of a softmax/sigmoid function, the corresponding sensitivity $\Delta = 1$. We can then leverage Gaussian or Laplace mechanism to add noise to the prediction scores. The corresponding results can be seen in Table ~\ref{tab:laplace_dp_for_prediction_score_criteo}. We can observe that the utility of the computed AUC is highly sensitive to the privacy budget. We cannot achieve a reasonable AUC utility with a small $\epsilon$ (i.e. $\epsilon \le 10$). 

 \input{tables/laplace_dp_for_prediction_score_criteo}

To achieve both privacy and utility, we can leverage the secure multi-party computation (MPC) technique ~\cite{mpc2011,mpc2012} to achieve the sorting goal. For example,  Hamada et al. ~\cite{mpc2012} constructed a quicksort protocol from the quicksort algorithm with their MPC sorting protocol. The resultant protocol can sort $32$-bit words and $1, 000, 000$ secret-shared values in $1, 227$ seconds, while existing sorting protocols cannot sort within $3, 600$ seconds.

In this paper, we adopt the vanilla setting to describe our AUC computation technique by default, since the prediction scores are shared between the server and clients. MPC based sorting protocol can replace our vanilla sorting method if necessary (privacy of prediction scores is a concern). 

\section{Figure: ~\ref{fig:dist_of_local_beta}: Distribution of local $\beta$}
\label{sec:dist_of_local_beta}

The distribution of local $\beta$ is shown in Figure ~\ref{fig:dist_of_local_beta}.

\begin{figure*}[ht!]
% \vspace{-0.1in}
\captionsetup[subfigure]{labelformat=empty}
  \begin{subfigure}{0.49\linewidth}
  \centering
    \includegraphics[width=1.0\linewidth]{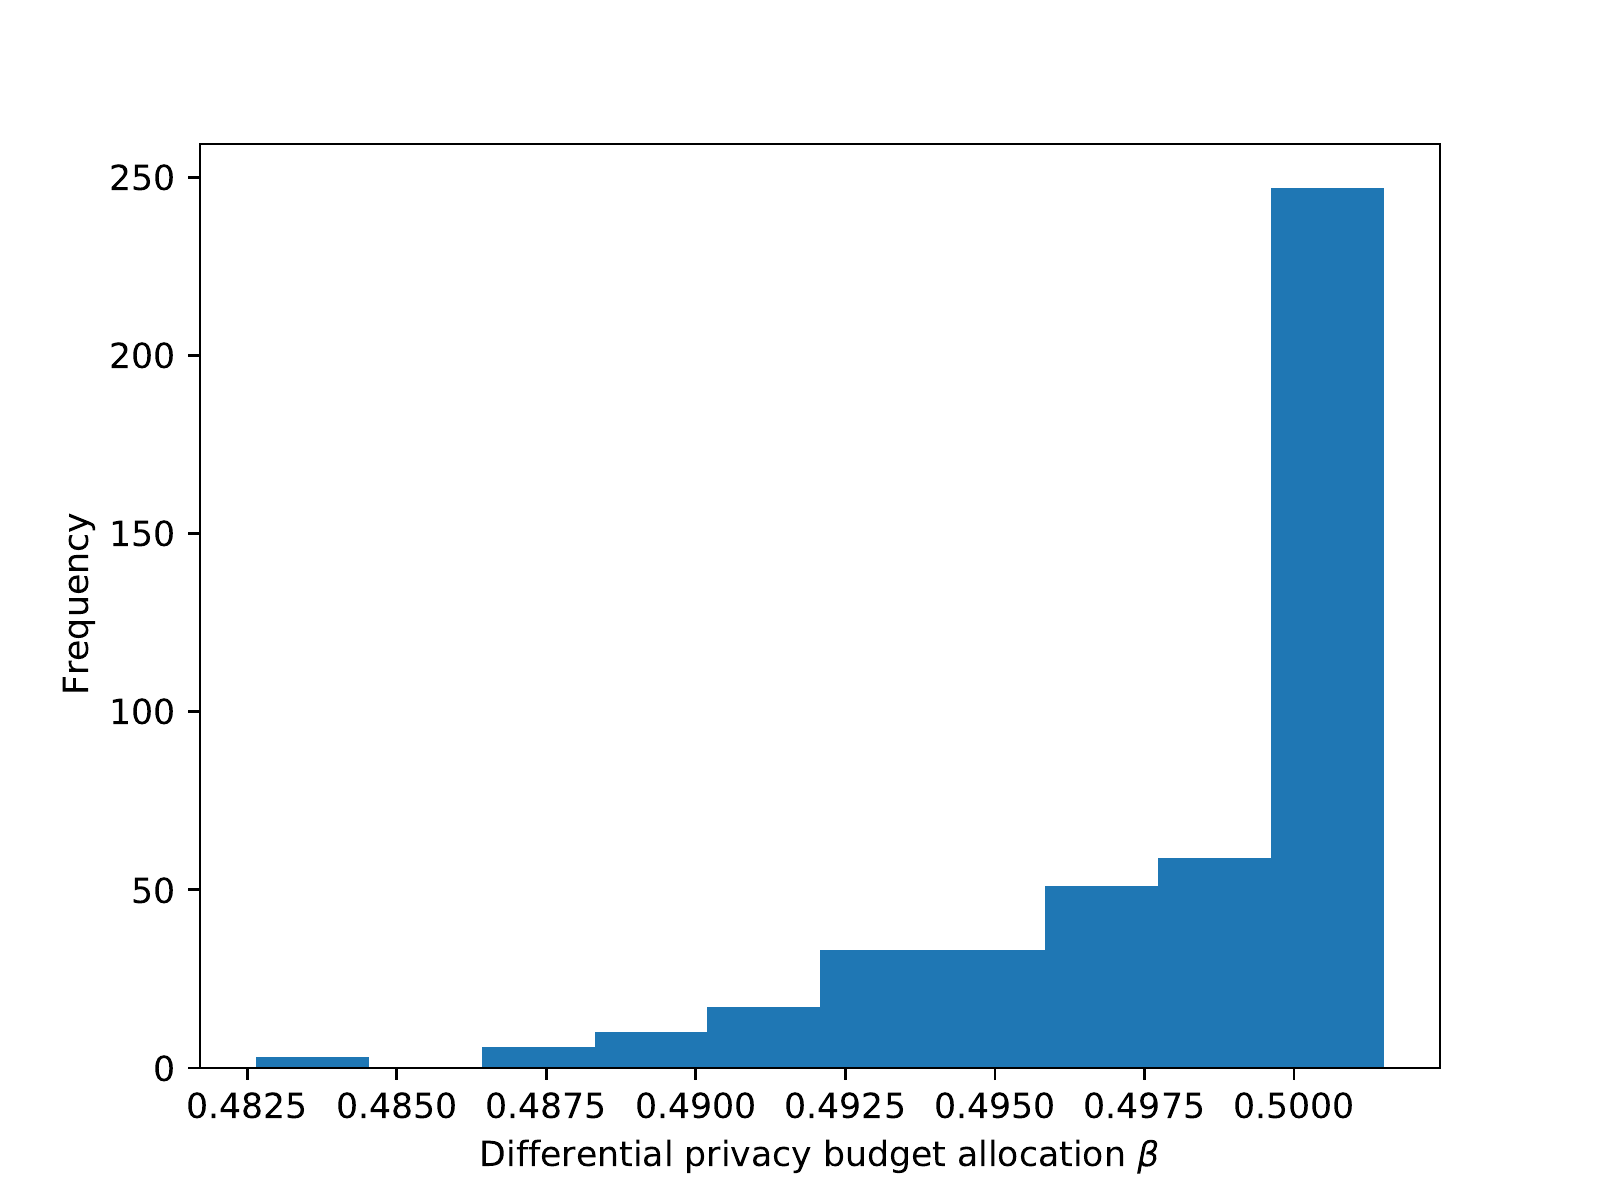}
      \caption{(a): Distribution of local $\beta$ in the IID setting. }
  \end{subfigure}
  \begin{subfigure}{0.49\linewidth}
  \centering
    \includegraphics[width=1.0\linewidth]{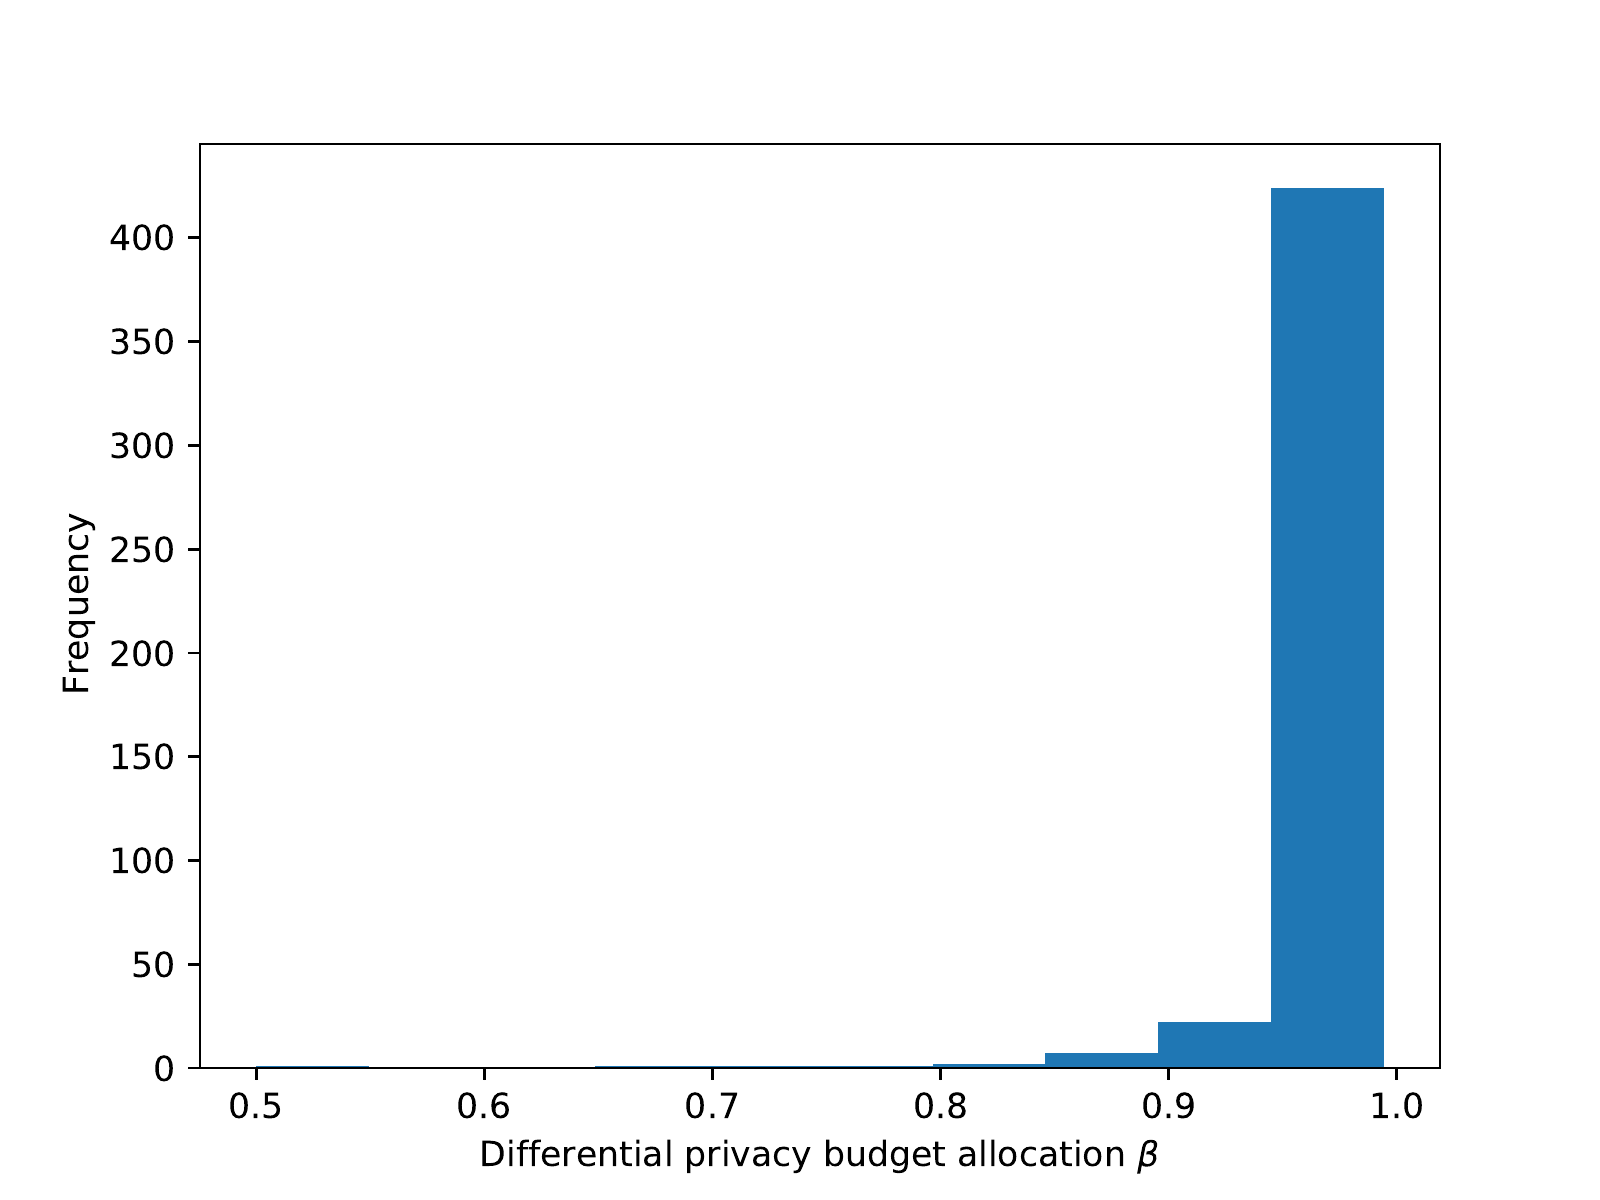}
    \caption{(b): Distribution of local $\beta$ in the Non-IID setting.}
  \end{subfigure}
  
   \caption{Distribution of local $\beta$}
 \label{fig:dist_of_local_beta} 
 \end{figure*}

\section{Computation resources}
\label{sec:computation_resources}

We conduct our experiments over a Macbook Pro with 2.4 GHz 8-Core Intel Core i9 and 64 GB 2667 MHz DDR4. Each epoch of run of Criteo takes about 2.5 minutes.
