# Supplementary material for: DPAUC: Differentially Private AUC Computation in Federated Learning
Source: arXiv:2208.12294 source file (2022-12-07)
Supplement: Supplementary file 3 [file appendix.tex]

\section{Algorithm of \ourapplap{}}
\label{sec:algorithm_dpauc_lap}
