# Supplementary material for: DPAUC: Differentially Private AUC Computation in Federated Learning
Source: arXiv:2208.12294 source file (2022-12-07)
Supplement: Supplementary file 4 [file auc_prob_view.tex]

\section{Computing  AUC from a probabilistic perspective}
\label{sec:auc_probabilistic_view}

In a binary classification problem, given a threshold $\theta$, a predicted score $s_i$ is predicted to be $1$ if $s_i \ge \theta$. Given the ground-truth label and the predicted label (at a given threshold $\theta$), we can quantify the accuracy of the classifier on the dataset with True positives (TP($\theta$)), False positives (FP($\theta$)), False negatives (FN($\theta$)), and True negatives (TN($\theta$)). Area under the Receiver operating characteristic (ROC) curves plots two variables: True Positive Rate (TPR)
 False Positive Rate (FPR). TPR (i.e. recall) is defined as $TPR(\theta) = \frac{TP(\theta)}{TP(\theta) + FN(\theta)}$. False Positive Rate (FPR) is defined as $(\theta) = \frac{FP(\theta)}{FP(\theta) + TN(\theta)}$.

\begin{itemize}
    \item True positives, TP($\theta$), are the data points in test whose true label and predicted label equals $1$. \textit{i.e.} $y_i = 1$ and $s_i \ge \theta$
    \item False positives, FP($\theta$), are the data points in test whose true label is $0$ but the predicted label is $1$. \textit{i.e.} $y_i = 0$ and $s_i \ge \theta$.
  \item  False negatives, FN($\theta$), are data points whose true label is $1$ but the predicted label is $0$. \textit{i.e.} $y_i = 1$ and $s_i < \theta$. 
  \item True negatives, TN($\theta$), are data points whose true label is $0$ and the predicted label is $0$. \textit{i.e.} $y_i = 0$ and $s_i < \theta$. 
\end{itemize}

% We will use the notation TP($\theta$), FP($\theta$), etc. to both denote the set of corresponding data points as well as the cardinality of these sets.

The ROC curve is defined by plotting  pairs of FPR($\theta$) (x-axis) versus TPR($\theta$) (y-axis) over all possible thresholds $\theta$. ROC curve starts at $(0,0)$ and ends at $(1,1)$. The area under the ROC curve (AUC) is used to evaluate the performance of a binary classifier. If the classifier is good, the ROC curve will be close to the left and upper boundary and AUC will be close to $1.0$. On the other hand, if the classifier is poor, the ROC curve will be close to  line from $(0,0)$ to $(1,1)$ with AUC around $0.5$.

\subsection{Computing AUC with Time Complexity O(PN)}

Area under ROC curve (AUC) is well studied in statistics and is equivalent to Mann-Whitney U statistics ~\cite{AUCProb2002,dpforclassifierEvaluation}. We focus on computing the AUC by 
 viewing it as the probability of correct ranking of a random positive-negative pair. Suppose we have $M$ samples including $P$ positives and $N$ negatives, where $M = P + N$. Given a classifier $\mathcal{F}$, it gives a prediction score $s_i$ for each sample $i \in [1, M]$. We then have $MN$ positive-negative pairs with score $<s_i, s_j>$ ($i \in [1, M]$ and $j \in [1, N]$) where $s_i$ and $s_j$ are prediction scores of positive sample $i$ and negative sample $j$ respectively. Then AUC of classifier $\mathcal{F}$ is:

\begin{equation}
    \text{AUC} = \frac{I(<s_i, s_j>)}{MN}, i \in [1, M] \quad \text{and} \quad j \in [1, N]
\end{equation}

where 
\begin{equation*}
    I(<s_i, s_j>) = \begin{cases}
                    1,  \text{if} \quad s_i > s_j,\\
                    0, otherwise.
                    \end{cases}
\end{equation*}

The time complexity of computing AUC is $O(PN)$.

\subsection{Computing AUC with Time Complexity $O(M \log M)$}
\label{sec:computing_auc_ranking}

We firstly rank all instances based on their prediction scores in an increasing order. Each score $s_i$ ($i \in [1, M]$) will be assigned a ranking $r_i$. The instance with the highest order will be assigned $r = M - 1$, and the second highest one will be assigned $M -2$ and so on. The smallest ranking score is $r = 0$.

Then AUC can be computed as:

\begin{equation}
\label{eq:auc_ranking_appendix}
    \text{AUC} = \frac{\sum_{i=1}^{M} r_i \cdot y_i - \frac{P(P-1)}{2} }{PN}
\end{equation}

where $y_i \in \{0, 1\}$ is the ground-truth label for instance $i$ (with ranking score $r_i$). The time complexity of this method is $O(M\log M)$.
