# Supplementary material for: DPAUC: Differentially Private AUC Computation in Federated Learning
Source: arXiv:2208.12294 source file (2022-12-07)
Supplement: Supplementary file 5 [file dist_of_beta.tex]

\begin{figure*}[ht!]
% \vspace{-0.1in}
\captionsetup[subfigure]{labelformat=empty}
  \begin{subfigure}{0.49\linewidth}
  \centering
    \includegraphics[width=1.0\linewidth]{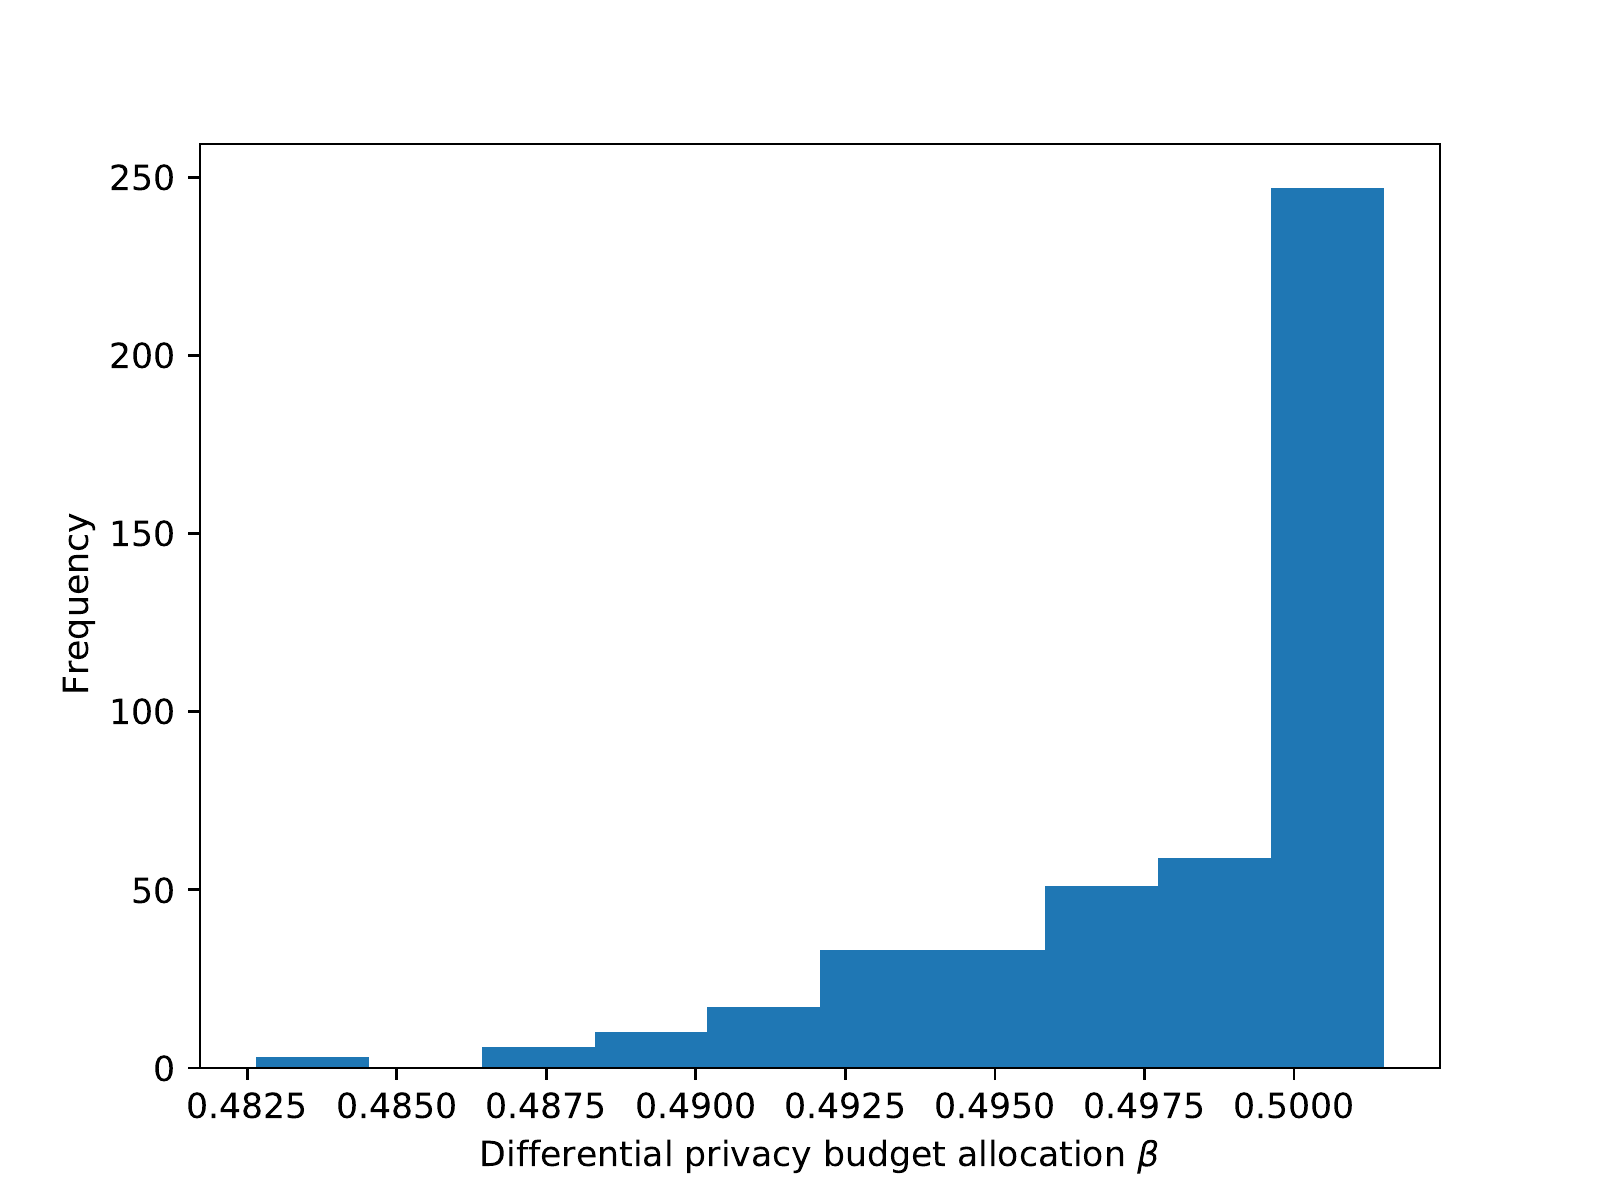}
      \caption{(a): Distribution of local $\beta$ in the IID setting. }
  \end{subfigure}
  \begin{subfigure}{0.49\linewidth}
  \centering
    \includegraphics[width=1.0\linewidth]{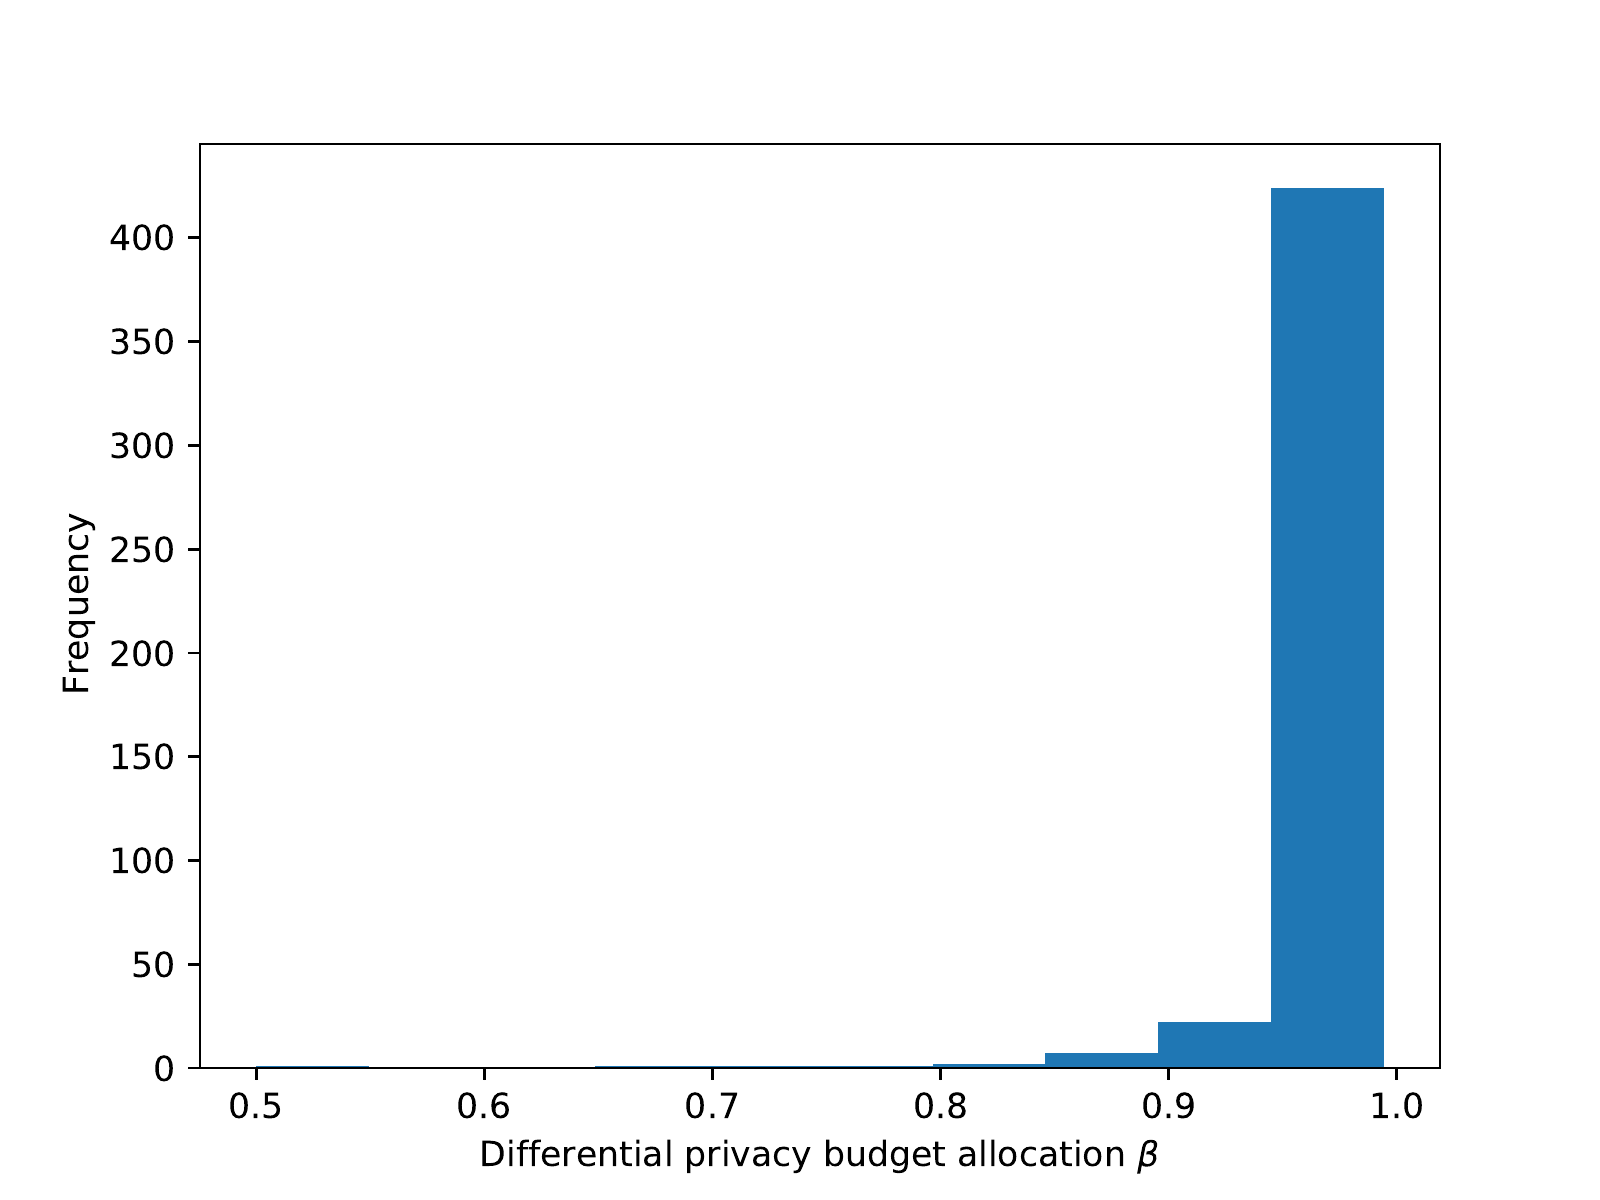}
    \caption{(b): Distribution of local $\beta$ in the Non-IID setting.}
  \end{subfigure}
  
   \caption{Distribution of local $\beta$}
 \label{fig:dist_of_local_beta} 
 \end{figure*}
