# Supplementary material for: DPAUC: Differentially Private AUC Computation in Federated Learning
Source: arXiv:2208.12294 source file (2022-12-07)
Supplement: Supplementary file 7 [file sorting_module.tex]

\section{Privacy Analysis of Prediction Scores}
\label{sec:sorting_module} 

In this section, we talk about how clients know the ranking results of their prediction scores and the corresponding privacy issue. 

In the vanilla setting, each client $C_k$ can send its shuffled prediction scores $s^k$ to the server. The server then aggregates all the prediction scores and sort them in an increasing order. Each prediction score $s_i^k$ ($i \in [1, M]$) will be assigned a ranking order $r_i^k$. The instance with the highest order will be assigned $r = M - 1$, and the second highest one will be assigned $M -2$ and so on. The smallest ranking score is $r = 0$. The server sends each ranking order $r_i^k$ back to the corresponding client $C_k$ which owns $s_i^k$. 
It's worth mentioning the prediction scores have to be shared with the server for some tasks. For example, the clients have to report the predicted conversion rate (CVR) of the ad impression to the server in online advertisements. The server \footnote{ad exchange} can later on calculate the bid price by multiplying the predicted CVR with  a constant parameter tuned according to the campaign budget and performance ~\cite{bidding2018}. Then the server can select the advertiser who proposed the highest bid price as the winner to show the ad.

\input{tables/top_k_analysis_criteo_data}

 \begin{figure}[ht!]% \vspace{-0.1in}
  \centering
    \includegraphics[width=0.75\linewidth]{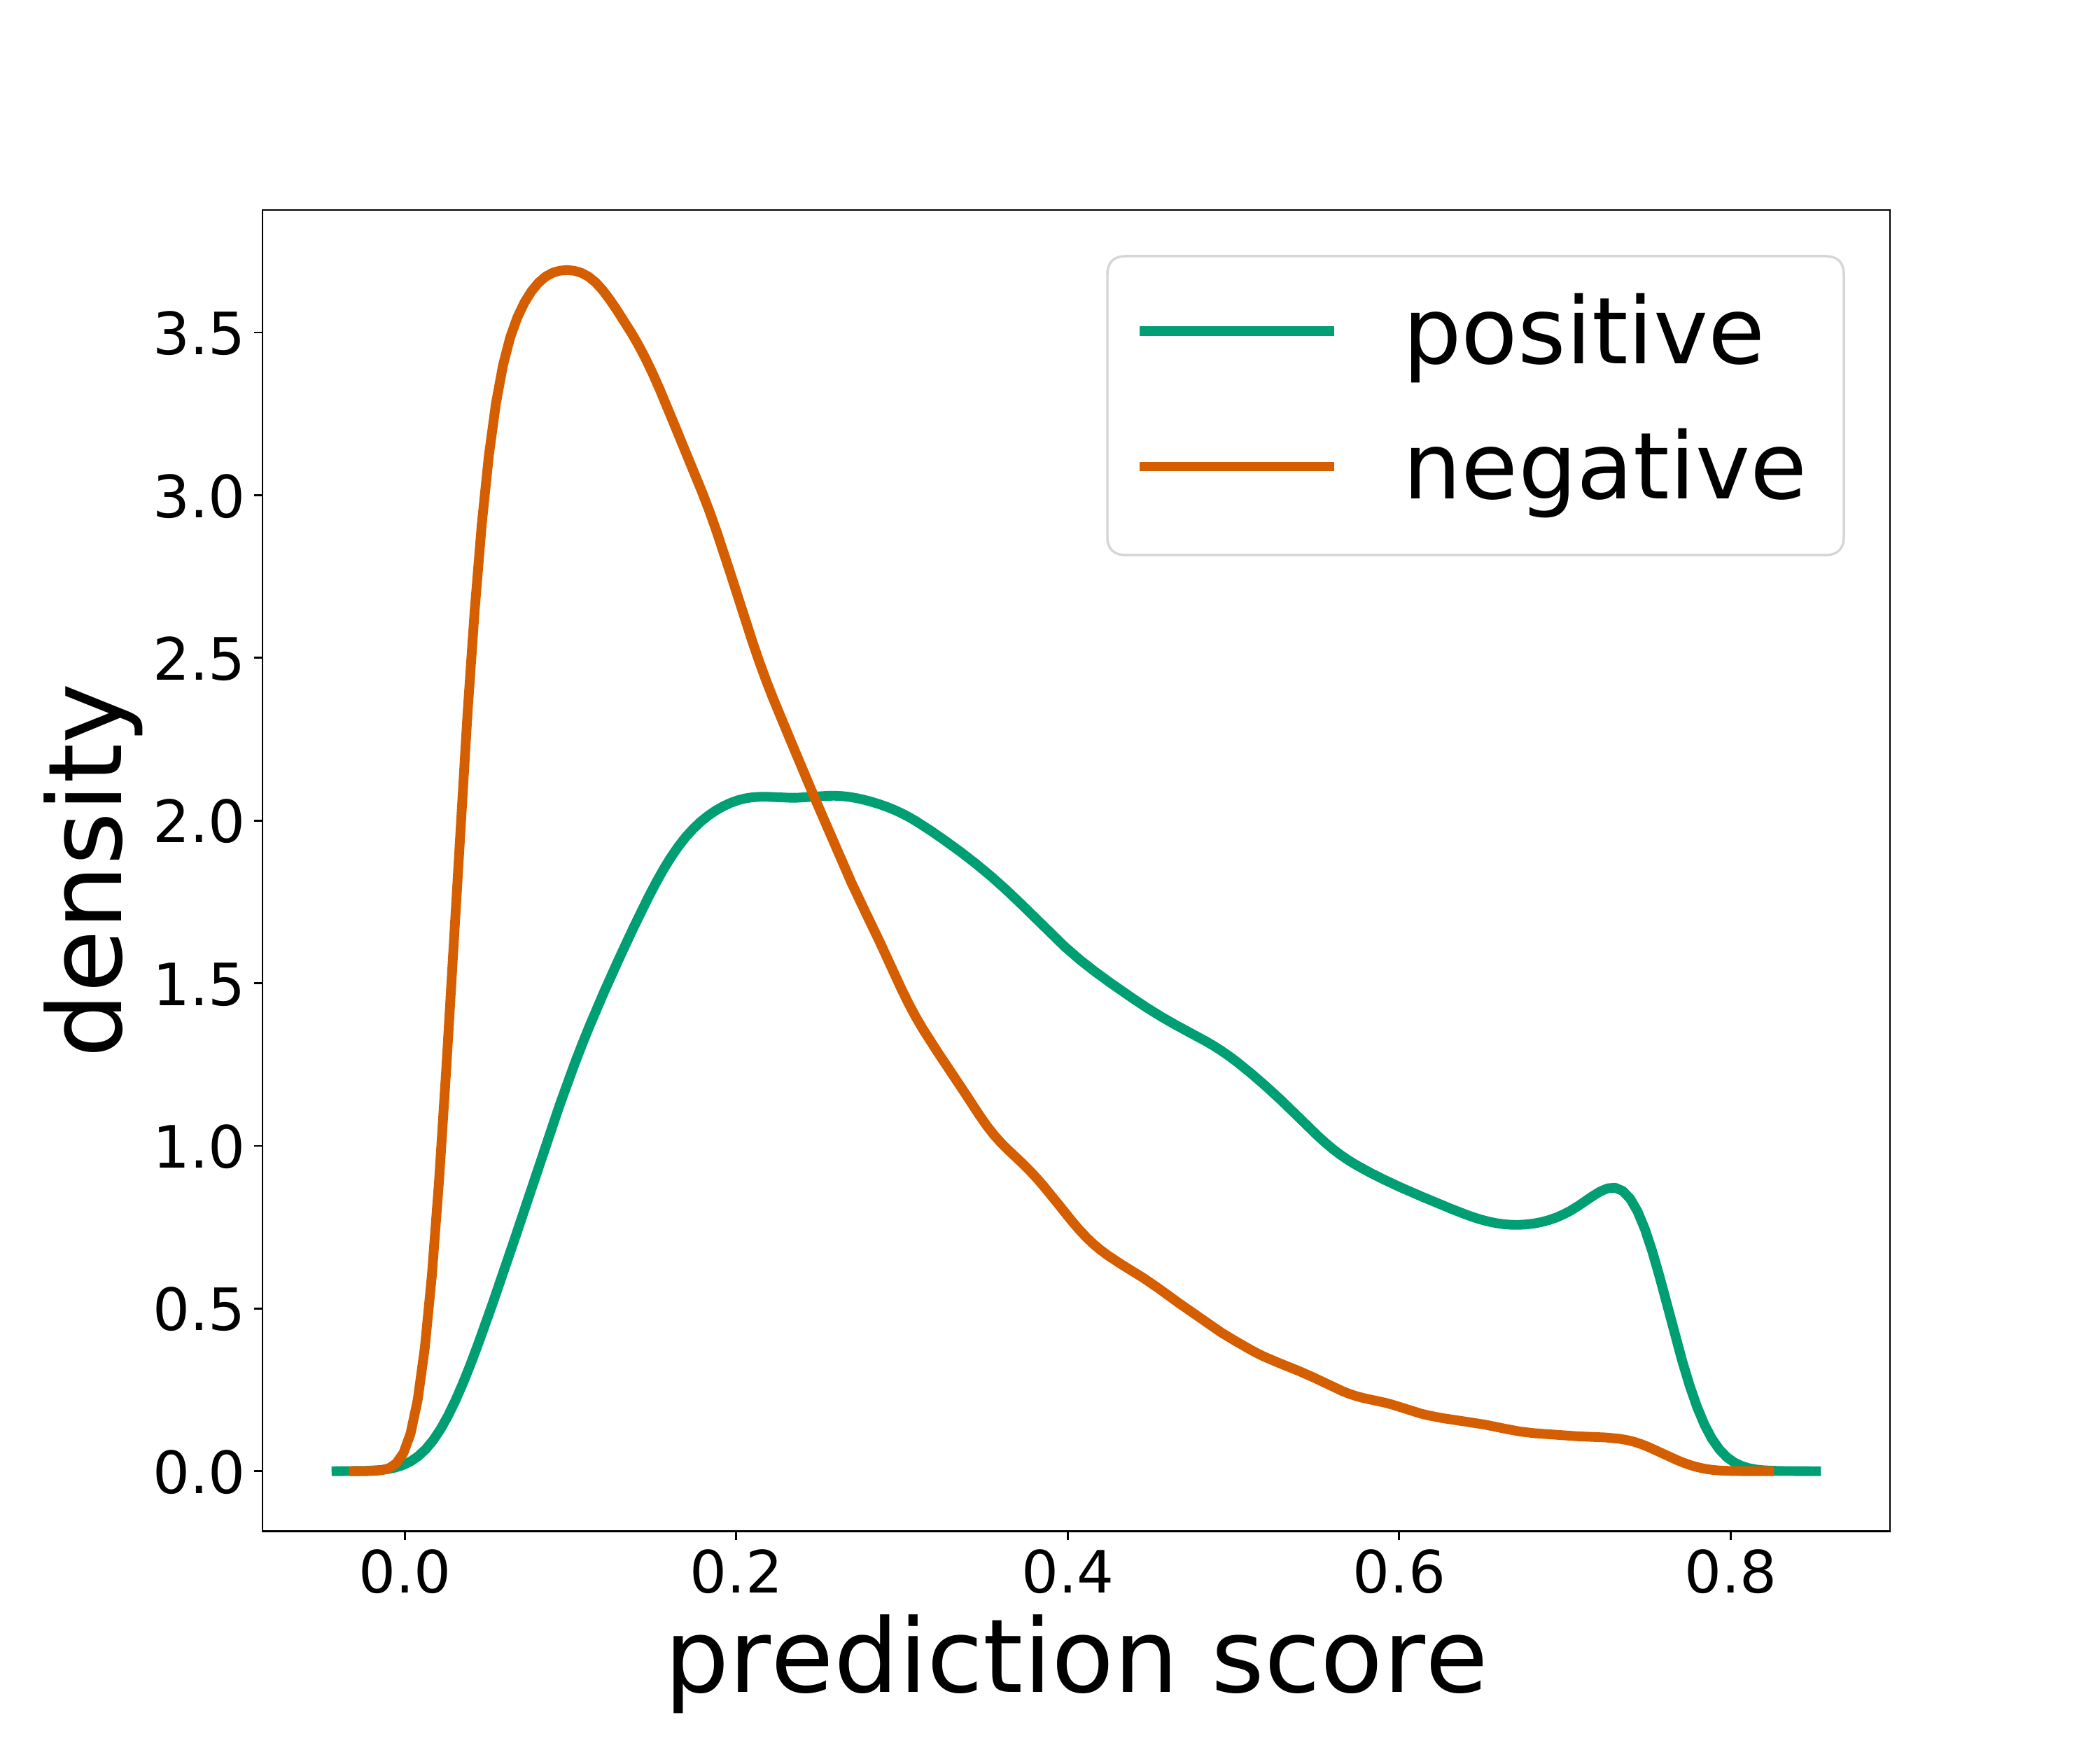}
  \caption{Density of positive and negative instances' prediction scores in Criteo data.}
 \label{fig:criteo_negative_positive_density} 
 \end{figure}

Interested readers may be curious if is it possible to infer the label information based on the prediction scores. Here we propose a simple attack method by selecting the samples with top-K prediction scores as positive labels. We measure the corresponding guessing performance by precision and recall. As shown in Figure ~\ref{fig:criteo_negative_positive_density} and Table ~\ref{tab:top_k_analysis_criteo_data_small}, positive instances can have a relative higher prediction scores than negative ones at some density areas. For example, we can achieve a $79\%$ precision if we select the instances with top-$100$ prediction scores. However, since the prediction scores $s^k$ are shuffled before sending to the server so that the server has no idea which prediction score belongs to which data sample \footnote{$|s^k| \geq 2$}. 

Instead of the vanilla setting, we also propose some alternative solutions to achieve the sorting goal. We may leverage DP to add noise to the prediction scores. Since the prediction score is the output of a softmax/sigmoid function, the corresponding sensitivity $\Delta = 1$. We can then leverage Gaussian or Laplace mechanism to add noise to the prediction scores. The corresponding results can be seen in Table ~\ref{tab:laplace_dp_for_prediction_score_criteo}. We can observe that the utility of the computed AUC is highly sensitive to the privacy budget. We cannot achieve a reasonable AUC utility with a small $\epsilon$ (i.e. $\epsilon \le 10$). 

 \input{tables/laplace_dp_for_prediction_score_criteo}

To achieve both privacy and utility, we can leverage the secure multi-party computation (MPC) technique ~\cite{mpc2011,mpc2012} to achieve the sorting goal. For example,  Hamada et al. ~\cite{mpc2012} constructed a quicksort protocol from the quicksort algorithm with their MPC sorting protocol. The resultant protocol can sort $32$-bit words and $1, 000, 000$ secret-shared values in $1, 227$ seconds, while existing sorting protocols cannot sort within $3, 600$ seconds.

In this paper, we adopt the vanilla setting to describe our AUC computation technique by default, since the prediction scores are shared between the server and clients. MPC based sorting protocol can replace our vanilla sorting method if necessary (privacy of prediction scores is a concern).
