# Supplementary material for: DPAUC: Differentially Private AUC Computation in Federated Learning
Source: arXiv:2208.12294 source file (2022-12-07)
Supplement: Supplementary file 8 [file utility_analysis_of_locallaplace.tex]

\section{Utility analysis of LocalLaplace}
\label{sec:utility_analysis_locallap_appendix}

To simplify the analysis, we assume that $P$ and $N$ are accurate\footnote{only adding noise to $\text{localSum}$} and each client only has one data sample\footnote{$\text{sum}_i \in [1, K-1]$}, the standard deviation of computed AUC by \locallap{} is:

\begin{equation}
\label{eq:var_locallap}
   \textbf{Var} (\text{AUC}_{\text{\locallap{}}})  =  \textbf{Var}(\frac{\sum_{i=1}^K sum_i}{P  N}) =  \frac{\sum_{i=1}^{K-1} 2*i^2 / \epsilon^2}{P^2  N^2} = \frac{K(K-1)(2K-1)}{3P^2  N^2  \epsilon^2}
\end{equation}
